# Supplementary material for: Carbon emissions and sustainability of launching 5G mobile networks in China
Source: arXiv:2306.08337 source file (2023-06-14)
Supplement: Supplementary file 1 [file Nature_Green_supplementary_material.pdf]

# Supplementary Information for Carbon Emissions and Sustainability of Launching 5G Mobile Networks in China

## SUPPLEMENTARY NOTE 1. MISALIGNMENT MEASUREMENT OF INFORMATION FLOW AND ENERGY FLOW

Network energy is not directly proportional to carried traffic load in mobile networks. An example presented in Fig. S6 is based on network traffic data collected from Nanchang, showing the total energy consumed versus the total traffic load. Even with almost no traffic, the total energy consumption is still relatively high at approximately 25.6 MWh. In contrast, the green dashed line in the figure depicts the desired energy consumption, which is proportional to traffic volume. The green star point in the figure denotes the $(C, E_{Max})$ point, where $C$ represents network capacity, which is the maximum amount of traffic the mobile network can support. $E_{Max}$ represents the maximum energy consumed when the carried traffic reaches the available capacity $C$. Given $(L, E)$, where $L$ represents the traffic load, and $E$ denotes the corresponding energy consumption in the real-world network, we then define the misalignment of energy between the real and desired cases as follows,

$$M^{Energy} = E - \frac{E_{Max}}{C} \cdot L, \tag{S1}$$

where $M^{Energy}$ denotes the misalignment of energy and $\frac{E_{Max}}{C} \cdot L$ represents the desired energy consumption under a traffic load of $L$. We then have,

$$M^{Energy} \propto \tilde{E} - \tilde{L}, \tag{S2}$$

where $\tilde{E} = E/E_{Max}$ represents the normalized energy consumption and $\tilde{L} = L/C$ represents the normalized traffic load. We then define $M = \tilde{E} - \tilde{L}$ as the **misalignment factor** between traffic load and energy consumption, which lies within the interval $[0, 1]$. The main factor causing this misalignment is that each base station's cooling power and fixed radio transmission overhead are unaffected by traffic load.

The relationship between energy efficiency and misalignment factor is then illustrated. In our case, energy efficiency is defined as the amount of network traffic that can be delivered per unit of energy consumption.

$$\eta^{Energy}(L) = L/E, \tag{S3}$$

where $\eta^{Energy}(L)$ denotes the energy efficiency under a traffic load of $L$. We then have,

$$\eta^{Energy}(L) = \frac{L}{E_{Max} \cdot M + \frac{E_{Max}}{C} \cdot L}. \tag{S4}$$

By denoting $C/E_{Max}$ as $\eta^{Energy}_{Desired}$, which represents the desired energy efficiency (the green dashed line in Fig. S6), we can derive the following expression,

$$\eta^{Energy}(L) = \frac{\eta^{Energy}_{Desired}}{1 + M/\tilde{L}}. \tag{S5}$$

Due to the misalignment between traffic load and energy consumption, the mobile network cannot achieve the desired energy efficiency. By reducing the misalignment factor, we can increase energy efficiency and mitigate both the energy and carbon efficiency traps.

## SUPPLEMENTARY NOTE 2. ENERGY CONSUMPTION MODEL OF BASE STATIONS

Base stations are fundamental components and consume the largest part of energy in mobile networks [1]. Figure S7 depicts a typical mobile network base station. A base station comprises a communication subsystem and a support subsystem. The Remote Radio Unit (RRU) and Base Band Unit (BBU), major components of the communication subsystem, are responsible for transceiving radio signals and processing baseband signals, respectively. A base station (BS) may have multiple RRUs and BBUs. The cooling and other auxiliary devices are part of the supporting subsystem. The cooling equipment, such as air conditioning, is used to maintain the proper operating temperature of the base station.

According to a base station's components, the overall power consumption $P_{BS}$ of a base station can be given by,

$$P_{BS} = P_{tx} + P_{cooling}, \tag{S6}$$

where $P_{tx}$ denotes the power consumption of the communication subsystem, and $P_{cooling}$ accounts for the power consumed by cooling equipment to maintain an appropriate operating temperature.

### Modeling Power Consumption of Communication Subsystem

The communication subsystem power consumption of a single base station is dominated by two components: RRU and BBU.

$$P_{tx} = P_{BBU} + P_{RRU}, \tag{S7}$$

where $P_{BBU}$ and $P_{RRU}$ represent the power consumed by BBUs and RRUs. Specifically, $P_{RRU}$ varies according to the base station traffic amount. When the traffic load is heavy, RRU has to consume more power to support more active physical resource blocks (PRBs)[1]. Thus, $P_{RRU}$ increases proportionately to traffic volume, i.e., the number of resource blocks utilized. In contrast, BBUs are responsible for baseband processing. No matter how many RBs are active, their power consumption remains relatively constant and is not affected by traffic load. By analyzing real-world data, we find that the BBU power of a base station is related to the number of cells it has. Generally, base stations with more cells have more BBUs. Fig. S8 shows the BBU power distribution for different types of BSes with different cell numbers. In real-world networks, there are three types of BSes in terms of their number of cells and network types: 4G BS with three cells, 5G BS with three cells, and 5G BS with six cells. Table S20 illustrates the average and standard deviation of the BBU power of various base stations. Since the BBU power of a particular BS type is mainly distributed in a small interval ($\pm$8.88%), we use the average value to approximate it. Specifically, for a 4G BS with three cells, its BBU power is simulated as 89.3771 W. For a 5G BS with three cells, its BBU power is simulated as 305.0409 W. For a 5G BS with six cells, its BBU power is simulated as 499.6484 W.

We next model the power consumption of RRUs $P_{RRU}$. Using measurement data on real-world mobile networks, we find that linear models can approximate a variety of base stations reasonably well; this model has been widely used in the literature [2–4]. Figure S9(a) and Figure S11(a) illustrate the scatter plots of RRU power $P_{RRU}$ and transmit power $P_{trans}$ in 4G and 5G networks, respectively. $P_{RRU}$ varies from 200W to 1200W. The relationship between RRU power and transmit power is strong and linear (Figure S10 and Figures S11(b) S11(c) S11(d)).

$$P_{RRU} = \alpha \cdot P_{trans} + \gamma, \tag{S8}$$

where $\alpha$ and $\gamma$ denote slope and offset, respectively. Notably, base stations of different settings[2], e.g., maximum transmit power, have specific coefficients in the linear regression model, as depicted in Table S21(a) and Table S22(a).

We then discover that transmit power varies with the physical resource block (PRB) usage ratio. The PRB usage ratio is the proportion of the base station's total available PRBs currently in use, reflecting the traffic load of a base station. Figure S12 and Figure S14(a) display scatter plots of transmit power and PRB usage ratio based on measurements from real-world mobile networks. $P_{trans}$ ranges between 0W and 300W. Given the same PRB ratio, the transmit power of 5G base stations is typically greater than that of 4G base stations because 5G base stations are equipped with more antennas[3]. Scatter plots clearly show that a linear model can approximate the transmit power with respect to the PRB usage ratio,

$$P_{trans} = \beta \cdot r_{_{PRB}} + \sigma, \tag{S9}$$

[1] A physical resource block (PRB) is the smallest unit of resources allocated to a mobile user for accessing cellular networks.
[2] As for 5G base stations, different base station types have specific settings for maximum transmit power (Figure S9(b)).
[3] 5G base stations are typically equipped with 32 or 64 antennas, whereas 4G base stations only have 4 or 8 antennas

where $r_{PRB}$ is the PRB usage ratio, $\beta$ and $\sigma$ denote slope and offset, respectively. As depicted in Table S21(b) and S22(b), base stations of different settings also have different coefficients. Notably, compared to 4G base stations, 5G base stations utilize an advanced technology known as subframe silence [5], in which transmit hardware is turned off when the subframe has no data to send. Consequently, the offset $\sigma$ of 5G base stations equals 0. In other words, there is no transmit power when there is no traffic load.

**RRU Power under Sleep Mode.** In order to conserve energy, it is common for mobile networks to switch base stations into low-power operational modes when the traffic load is extremely low by turning off some RRU components, such as the power amplifier. These low-power modes are referred to as sleep modes. When a base station is in sleep mode, its RRU power becomes independent of traffic load. We then plot the cumulative distribution function (CDF) of RRU power in sleep mode based on real-world measurement data. Fig. S15 shows that the RRU power of 5G base stations in sleep mode is typically lower than that of 4G base stations, owing to the advanced physical Energy-saving technology utilized by 5G mobile networks [6]. In our case, we then approximate the RRU power in sleep mode based on the mean value of the various base station types. Table S23 illustrates the mean and standard deviation of RRU power in sleep mode for various base station types.

### Modeling Power Consumption of Supporting Subsystem

In this paper, we only model the power consumption of cooling devices, as they account for the vast majority of the total power consumption of the supporting system. In practice, the power consumption of the cooling devices can be simulated using EnergyPlus [7], a program developed by Lawrence Berkeley National Laboratory (LBNL). EnergyPlus can simulate how the power consumption of the cooling system fluctuates every half-hour by receiving as inputs the outdoor air temperature, the indoor proper operating temperature, the power generated by the communication subsystem, and the room area of the base station. Specifically, information on outdoor air temperature can be found in the World Meteorological Organization's weather dataset[4]. The communication subsystem is modeled as an electrical heat source. According to the 'Technical Standard for Mobile Communication Infrastructure of Construction' recognized by the Chinese government, we established a base station room with a $20m^2$ area and a 20°C proper operating temperature. The EnergyPluse parameter settings are displayed in Table S24.

[4] https://worldweather.wmo.int/en/home.html

## SUPPLEMENTARY NOTE 3. ESTIMATION OF RESIDENTIAL AND INDUSTRIAL POWER LOAD IN NANCHANG

We use two methods to estimate the residential and industrial power load $P_{orig}(t)$ in Nanchang: static approximation and dynamic approximation. In static approximation, $P_{orig}(t)$ is assigned as a constant annual mean value. According to [8], the total energy consumption of Nanchang city in 2020 is 25.399 billion KWh, which means the average power load is about 2891.5 MW, and thus $P_{orig}(t) = 2891.5$ MW. Due to the delay in the government's release of detailed power load data, we could only approximate the load in 2022 using the publicly available data for 2020. In dynamic approximation, we utilize the typical load patterns within one day and one year to more precisely approximate the power load of Nanchang. According to [9], the typical load curve in Jiangxi province within one year and one day is shown in Fig. S16. However, the exact values at each time are unknown. We next used the maximum, and minimum power load of Nanchang in 2020 [8] to estimate $P_{orig}(t)$ in every half-hour. Notably, $P_{Orig}(t)$ is assumed to be devoid of $P_{BS}(t)$. As depicted in Fig. S16 (a), there are two curves representing the maximum and minimum daily power loads, denoted as $P^{max}_{day}(k)$ and $P^{min}_{day}(k)$ for $k \in \{1, 2, ..., 366\}$. According to [8], the maximum and minimum power loads of Nanchang city in 2020 are 4650 MW and 1769 MW, respectively, denoted as $P^{max}_{year} = 4650$ MW, $P^{min}_{year} = 1769$ MW. Then, the specific daily values of $P^{max}_{day}(k)$ and $P^{min}_{day}(k)$ are computed as follows,

$$P^{max}_{day}(k) = P^{min}_{year} + r^{max}_{year}(k) * (P^{max}_{year} - P^{min}_{year}), \ \forall k \in \{1, 2, ..., 365\}, \tag{S10}$$

$$P^{min}_{day}(k) = P^{min}_{year} + r^{min}_{year}(k) * (P^{max}_{year} - P^{min}_{year}), \ \forall k \in \{1, 2, ..., 365\}, \tag{S11}$$

where $r^{max/min}_{year}(k)$ is the ratio of $(P^{max/min}_{day}(k) - P^{min}_{year})$ over $(P^{max}_{year} - P^{min}_{year})$, which can be obtained directly from the curve of Fig. S16 (a) without knowing the exact values. After obtaining $P^{max}_{day}$ and $P^{min}_{day}$ for each day, the detailed half-hourly power load within a day is computed based on the typical load curves for weekdays and weekends, as shown in Fig. S16 (b) and (c). Using the same methods as Eq. (S10) and Eq. (S11), $P_{orig}(t)$ for the $k$-th day is computed as follows,

$$P_{orig}(t) = P^{min}_{day}(k) + r_{day}(t) * (P^{max}_{day}(k) - P^{min}_{day}(k)), \ \forall t \in T, \tag{S12}$$

where $r_{day}(t)$ is the ratio of $(P_{orig}(t) - P^{min}_{day})$ over $(P^{max}_{day} - P^{min}_{day})$, which could also be obtained directly from the load curves of weekdays and weekends shown in Fig. S16 (b) and (c).

The above two methods (static approximation and dynamic approximation) to compute $P_{orig}(t)$ may result in different amounts of carbon emissions. To evaluate the difference between the two methods, we first calculated the carbon emissions of base stations using $P_{orig}(t)$ generated by the two methods without considering the PV power generation of base stations. As shown in Fig. S17 (a) and (b), the resultant mobile network carbon emissions using the two methods are the same during some time slots and also show significant differences during others. To determine why the number of carbon emissions using the dynamic approximation method drops sharply during certain time slots, we further show the dynamic load curve of $P_{orig}(t)$ in Fig. S17 (c), and the power generation of XinChang power unit 1 and 2 ($P_{1/2}(t)$) in Fig. S17 (c) and (d). XinChang power unit has a larger capacity with lower $c^{coal}_i$ than the other generation units. As shown in Fig. S17 (c), $P_{1/2}(t)$ essentially maintains maximum power generation (700MW) due to their lower $c^{coal}_i$; however, when $P_{orig}(t)$ continues to decrease at about 21:30 each day, $P_{1/2}(t)$ is eventually influenced and begins to decrease. In other words, the decrease in $P_{orig}(t)$ causes $P_{1/2}(t)$ to fall below their maximum capacity after 21:30. From Fig. S17 (d), which shows the additional power generation ($\Delta P_{1/2}(t)$) of XinChang power unit 1 and 2 for mobile network power load, it can be seen that, because $P_{1/2}(t)$ has low values between 21:30 and 7:00 of the following day, the two units with lower carbon emissions factors than the other units are able to provide their rest power capacity to the power load, and thus the carbon emissions amount caused by mobile network power load decreases sharply during that time. The dynamic approximation could demonstrate more realistic carbon emissions caused by mobile networks compared to the static approximation approach. As a result, the dynamic approximation method is applied to obtain $P_{orig}(t)$ in this work.

## SUPPLEMENTARY NOTE 4. ENERGY-SAVING METHODS

An Energy-saving method of mobile networks is to switch base stations (BSes) into low-power operational modes by turning off certain RRU components, such as the power amplifier, when the traffic load is extremely low. When a base station goes into sleep mode, its traffic will be handled by nearby active base stations. As illustrated in Fig. S18, when the PRB usage ratio (or traffic load) of base station A is low, base station A enters sleep mode, and the mobile user served is offloaded to adjacent base station B that is referred to as base station A's compensating base station. In particular, a base station is referred to as the compensating base station of another when its maximum communication range is sufficient to cover the normal communication range of another base station. In practice, Energy-saving methods control the working states of cells to determine whether cells enter sleep mode. A cell refers to a carrier on a sector of a base station. A base station generally has multiple cells.

### Threshold-based Method

Current mobile networks generally employ a threshold-based method. A cell will enter sleep mode when two conditions are met. The first condition is that it has at least one active compensating cell. The second condition is that its load, as determined by its PRB usage ratio and the number of users, is below a predetermined sleep threshold. Typically, sleep thresholds are established manually based on the knowledge of experts. Table S25 displays the parameter settings of the threshold-based method used in current real-world mobile networks.

### Greedy Method

The greedy method [2] is representative of the methods that use combinatorial optimization to optimize the working state of cells, which consists of two steps: grid-based partition and greedy selection of active cells.

#### *Grid-based Partition*

We partition the space into small grids based on the compensation relationships between cells, with equivalent cells in each grid. In our case, cells are equivalent if they can communicate with mobile users interchangeably. In other words, two cells are equivalent if they act as compensating cells for one another. When all cells inside are equivalent, a virtual grid is created. Once a cell is not equivalent to every cell in the existing grid, a new grid is created.

#### *Greedy Selection of Active Base Stations*

In order to reduce the misalignment of information flow and energy flow in mobile networks, we choose the appropriate set of active cells and put the rest into sleep mode based on the grid-based partition result. The selection must meet coverage and capacity[5] requirements. For a particular grid, we first identify the time of day with the highest network traffic based on the 24-hour traffic profile and then select the active set of cells for this peak time. Notably, in order to meet the coverage and capacity criteria, the local aggregate capacity of all active cells must be sufficient to handle local traffic. By doing so, the greedy selection algorithm favors cells with greater capacities. Consequently, we arrange each cell in the grid based on decreasing capacity values. The set of active cells is then chosen every half-hour based on the capacity order.

### DeepEnergy

Due to that, the total capacity is much larger than the total traffic demand in the system. We consider setting the control status of cells to sleep mode and reallocating the traffic for the active cells to save energy.

### Multi-Agent Collaboration Problem

There are three sub-tasks: base station control, cell control, and traffic allocation. Cell control is in the leading role. Once the cell control is obtained, the base station control and traffic allocation can be obtained by simple rules. We consider cell control as a multi-agent collaboration problem: each cell $c_n$ is managed by an agent $agent_n$, and these agents cooperate to minimize the energy consumption of the system. In this problem, agents output actions based on their observations (part of the system state), and these actions act together on the system. The system changes its state based on the joint actions and feeding back rewards to each agent.

[5] The maximum volume of traffic a cell can support is referred to as its capacity.

***Observation***

The observation of each agent $agent_n$ includes the feature vectors of other cells in the same base station or the same grid. The feature vector of cell $c_n$ consists of time $t$, the traffic loads of the grid $g_m$ that the cell $c_n$ belongs to in the last four time steps, $(L^m_{t-4}, L^m_{t-3}, L^m_{t-2}, L^m_{t-1})$, and the device parameters of the cells in $\mathcal{N}^g_m \cup \mathcal{N}^b_k$. $\mathcal{N}^g_m$ denotes the set of cells in the grid $g_m$ and $\mathcal{N}^b_k$ denotes the set of cells of the base station $BS_k$ that the cell $c_n$ belongs to.

***Action***

The optional action of an agent is setting its corresponding cell to the active or inactive status. The final decision of BSes, cell control, and traffic allocation is obtained based on the agents' decision by the following steps. Firstly, adjust the action output by the agents. If the total capacity of active cells in a grid is less than the traffic demand, the inactive cells would be activated from the largest to the smallest capacity until the total capacity of active cells is higher than the demand. Secondly, allocate predicted traffic on the active cells. The predicted traffic demand in the grid is divided according to the active cells' capacity and then assigned to the corresponding cells. Finally, obtain the control status of BSes and cells. If all cells in a base station were inactive, DeepEnergy would turn off the base station and its cells. Otherwise, the control status of that base station is set to turn on, and the cell's status is set to open (sleep) if its status is active (inactive).

***Reward***

The decisions aim to save the total energy, including the RRUs, BBUs, and air conditioners. The reward should encourage the agents to cooperate to save energy consumption. When the control states of other cells remain unchanged, the change of the control status of a cell can only affect the energy consumption in the base station it belongs to and the grid it belongs to. Thus, the reward for each agent is set to $r_n = -\sum_{n' \in \mathcal{N}^g_m} P^{RRU}_{n'} - P^{BBU}_k - P^{cooling}_k$. The first term indicates the energy of RRUs in cells that belong to the same grid as cell $c_n$, so it could encourage the agent to cooperate with agents from these cells $\{c_{n'}\}_{n' \in \mathcal{N}^g_m}$. The second term indicates the energy of BBUs and cooling devices in the base station that cell $c_n$ belongs to, which may encourage the agent to cooperate with the agents from the same base station.

## Local Collaboration-based Cell Control

***Overview***

To solve this multi-agent collaboration problem, we consider training a policy network to output the action based on the current state. A large number of agents is a major challenge. On the one hand, the large-scale agents lead to a massive state space, so when an agent makes the decision, it should efficiently integrate the state of other agents associated with it. For this problem, we construct two graphs based on the intra-grid and intra-BS relationships and then use the graph neural network to integrate the information of the associated nodes in the graphs. On the other hand, large-scale agents also lead to complex interactions between agents, making the expected rewards of different actions difficult to estimate. Thus, we introduce the idea of Mean-Field MARL (MF-MARL [10]) to integrate the effects of other agents' decisions on the target agent and design two masks to decrease the difficulty of action value estimation. In the following, we will build a graph for the relationship among cells, construct a graph neural network-based action value network, and describe how to train the network.

***Action-value Network Architecture***

Action-value network architecture is as follows: For a cell $c_n$ and its agent, the capacity and device parameters of each cell associated with $c_n$ are embedded in two linear layers. The embeddings of cells from the same grid (or base station) as $c_n$ are integrated by an attention layer. The two integrated embeddings, global values (such as time step and traffic demand in the grid), and masks are concatenated into a single vector, which is then fed into two fully connected layers to produce the final output. The final output is the predicted reward for different actions. The architecture, as mentioned above, can effectively integrate local information from relevant cells with global information.

***Action-value Network Update***

We design an RL method similar to MF-MAR to train the action-value network. MF-MARL approximates the effect of the actions of all other agents (or neighborhood agents) with one of the averages of these actions. In other words, MF-MARL predicts the action value for an agent

depending on the system state, the agent's action, and the average action of all other agents (or neighborhood agents). In this problem, we replace the average of the actions with two masks which depend on the action of related agents and directly determine the agent's reward. The first mask denotes whether the grid's traffic demand could be met if the agent sets the respective cell to sleep. The second mask denotes whether all other cells under the same base station could sleep if the cell is set to sleep mode.

These masks are derived from the actions of other agents and can only be used as training input. Therefore, each agent has two action-value networks, $q^2(\mathbf{o}_n, a, \mathbf{m}_n; \theta_q^2)$ for training and $q^1(\mathbf{o}_n, a; \theta_q^1)$ for inference, where $\mathbf{o}$ denotes the observation, $a$ denotes the action, $\mathbf{m}$ denotes masks, and $\theta$ denotes the parameters of action-value networks. In the execution stage, the action-value network without masks as input, $q^1(\mathbf{o}_n, a; \theta_q^1)$, predicts the rewards associated with different actions, setting the cell to sleep or not, based on the observation. Using $\epsilon$-greedy method, the agent determines the status of the cell by sampling the action based on predicted rewards. After the statuses of all cells determined by the agents are executed, the rewards for all agents are calculated. All agents' observations, actions, and rewards are appended to the replay buffer. In the training stage, the action-value network with masks as input, $q^2(\mathbf{o}_n, a, \mathbf{m}_n; \theta_q^2)$, is trained with the replay buffer to predict the rewards of different actions based on the observation and masks. The network $q^2$ is optimized through the following loss function:

$$L_2 = \frac{1}{2}\left[q^2(\mathbf{o}_n, a, \mathbf{m}_n; \theta_q^2) - r_n\right]^2, \tag{S13}$$

where the masks $\mathbf{m}_n$ is obtained based on the actions recorded in replay buffer. The action-value network, $q^1(\mathbf{o}_n, a; \theta_q^1)$, is then optimized by imitating the second one, $q^2(\mathbf{o}_n, a, \mathbf{m}_n; \theta_q^2)$,

$$L_1 = \frac{1}{2}\sum_a \left[q^1(\mathbf{o}_n, a; \theta_q^1) - q^2(\mathbf{o}_n, a, \mathbf{m}_n; \theta_q^2)\right]^2, \tag{S14}$$

where the mask $\mathbf{m}_n$ are calculated based on the re-sampled actions, which is sampled as the process in the execution stage. The re-sampling process is equivalent to the sampling process for the distribution of the mask vector. Thus, the first network $q^1$ would learn to predict the rewards of various actions under the sampled distribution of the mask vector. The framework of DeepEnergy is shown in Fig. S19. The algorithm is shown in Algorithm S1.

**Algorithm S1.** DeepEnergy for Cell and Base Station Status Controlling.

**Require:** The cell IDs belonging to each grid $g_m$, $\mathcal{N}_m^g$, the cell IDs belonging to each base station $b_k$, $\mathcal{N}_k^b$ and the device parameters of the each cells $\{\mathbf{x}_n\}_{n=1}^N$
Initialization the action-value networks $q^1(\mathbf{o}_n, a; \theta_q^1)$ and $q^2(\mathbf{O}_n, a, \mathbf{m}_n; \theta_q^2)$
**while** training not finished **do**
  **for** $i \leftarrow 1$ to 48 **do**
    Utilize the action-value network $q^1(\mathbf{o}_n, a; \theta_q^1)$ to predict the value of different actions for each cell
    Sample the action $a^n$ based on the predicted value
    Get the traffic demands of all grids at timestep $t$
    Use the actions $\{a^n\}_{n=1}^N$ to adjust the control status of cells and base stations
    Calculate the energy consumption of each cell and each base station
    Calculate the reward for each agent, $r^n = -\sum_{n' \in \mathcal{N}_m^g} P_{n'}^{RRU} - P_k^{BBU} - P_k^{Air}$
    Store $< \{\mathbf{o}_n\}_{n=1}^N, \{a_n\}_{n=1}^N, \{r_n\}_{n=1}^N >$ to replay buffer
    **for** $j \leftarrow 1$ to $J$ **do**
      Sample a batch of samples from replay buffer
      Randomly select a cell for each sample, and calculate the mask for the cell
      Update the action-value network $q^2$ by minimizing the loss of S13
      Update the action-value network $q^1$ by minimizing the loss of S14

## Supplementary Note 5. Estimation of Misalignment Factor Across Provinces

The misalignment factor, denoted by $M = \tilde{E} - \tilde{L}$, measures the discrepancy between the normalized energy consumption ($\tilde{E}$) and the normalized traffic load $\tilde{L}$ in the mobile network. By analyzing real-world data without energy-saving and simulation results under different energy-saving methods conducted in Nanchang, we find that the misalignment factor of the mobile network varies with the normalized network traffic load and the energy-saving method it uses, as depicted in Fig. S20. Under a specific energy-saving scenario, the misalignment factor ($M$) linearly decreases as the normalized network traffic load ($\tilde{L}$) increases, and $M = 0$ when $\tilde{L} = 1$. Thus, we have

$$M = K_\psi(1 - \tilde{L}), \tag{S15}$$

where $K_\psi$ denotes coefficient and depends on the energy-saving scenario $\psi$. The linear regression model can approximate the misalignment factor with an R-squared of over 0.81 for various energy-saving scenarios (Fig. S21). Table S26 shows the coefficients for different energy-saving scenarios based on the data from Nanchang.

In our case, we assume that all provinces share the same coefficient $K_\psi$ with Nanchang under the energy-saving scenario $\psi$. Therefore, given the normalized traffic load $\tilde{L}_p$ of province $p$, we can estimate its misalignment factor $M_{p,\psi}$ under energy-saving scenario $\psi$ as,

$$M_{p,\psi} = K_\psi(1 - \tilde{L}_p). \tag{S16}$$

Notably, the normalized traffic load $\tilde{L}_p$ of province $p$ varies over time, and consequently, so does its misalignment factor $M_{p,\psi}$. Tables S27, S28, S29, and S30 illustrate the estimated misalignment factors for each province under various energy-saving scenarios.

## Supplementary Note 6. Generalizability Analysis of DeepEnergy

DeepEnergy is of a high generalizability because it utilizes mean-field MARL to integrate the effects of other agents' decisions on the target agent. To verify the generalizability of DeepEnergy, we partition Nanchang into four regions, according to the city center point. As depicted in Fig. S22, we denote them as Region A, Region B, Region C, and Region D. These four regions have different base station density, network capacities and network traffic loads. We then train DeepEnergy on the data from each of these four regions, and then apply the trained model from each region to the whole Nanchang to test its performance. Table S31 shows that the models trained on data from different regions have similar performance. Further, we use the performance results of the models trained on data from different regions to fit the relation between misalignment factor and the normalized network traffic load (Eq. S15). Different models have similar coefficient $K_\psi$, reflecting that they have similar energy-saving capabilities (Fig. S23 and Table S32). Consequently, DeepEnergy has high generalizability over different training data.

## REFERENCES


1. C.-L. I, S. Han, and S. Bian, "Energy-efficient 5G for a greener future," Nat. Electron. **3**, 182–184 (2020).
2. C. Peng, S.-B. Lee, S. Lu, H. Luo, and H. Li, "Traffic-driven power saving in operational 3G cellular networks," in *Proceedings of the 17th annual international conference on Mobile computing and networking,* (2011), pp. 121–132.
3. P.-H. Huang, S.-S. Sun, and W. Liao, "Greencomp: Energy-aware cooperation for green cellular networks," IEEE Transactions on mobile computing **16**, 143–157 (2016).
4. Q. Wu, X. Chen, Z. Zhou, L. Chen, and J. Zhang, "Deep reinforcement learning with spatio-temporal traffic forecasting for data-driven base station sleep control," IEEE/ACM Transactions on Netw. **29**, 935–948 (2021).
5. S. Rostami, K. Heiska, O. Puchko, K. Leppanen, and M. Valkama, "Pre-grant signaling for energy-efficient 5g and beyond mobile devices: Method and analysis," IEEE Transactions on Green Commun. Netw. **3**, 418–432 (2019).
6. D. López-Pérez, A. De Domenico, N. Piovesan, G. Xinli, H. Bao, S. Qitao, and M. Debbah, "A survey on 5G radio access network energy efficiency: Massive mimo, lean carrier design, sleep modes, and machine learning," IEEE Commun. Surv. & Tutorials **24**, 653–697 (2022).
7. D. B. Crawley, L. K. Lawrie, F. C. Winkelmann, W. F. Buhl, Y. J. Huang, C. O. Pedersen, R. K. Strand, R. J. Liesen, D. E. Fisher, M. J. Witte *et al.*, "Energyplus: creating a new-generation building energy simulation program," Energy buildings **33**, 319–331 (2001).
8. "Notice of the office of the people's government of nanchang city on forwarding the 2021 plan of the municipal development and reform commission and state grid nanchang power supply company for orderly power consumption of nanchang power grid," Tech. rep., Gazette of Nanchang Municipal People's Government (2021). http://www.nc.gov.cn/nc_xxgk/jsp/zfgb/ncgb_content.jsp?mid=a731211fe1094abfaea8ab348bd5ba8b.
9. "Notice on signing medium and long term power contracts in 2021," Tech. rep., National Development and Reform Commission/National Energy Administration (2021). http://www.gov.cn/zhengce/zhengceku/2020-12/03/content_5566580.htm.
10. Y. Yang, R. Luo, M. Li, M. Zhou, W. Zhang, and J. Wang, "Mean field multi-agent reinforcement learning," in *International conference on machine learning,* (PMLR, 2018), pp. 5571–5580.

## LIST OF FIGURES

S1 Launching 5G Leads to the appearance of energy efficiency trap in Nanchang. (a) The operation of newly launched 5G base stations has led to a sharp increase in energy consumption in Nanchang. (c) Launching 5G Leads to the appearance of an energy efficiency trap and causes extra energy consumption in Nanchang. . . . 13
S2 The daily energy consumption vs. the number of base stations. The energy consumption of a mobile network are highly correlated with its number of base stations. 14
S3 The spatial distribution of (a) normalized traffic loads of 4G networks, (b) normalized energy consumption of 4G networks, (c) normalized traffic loads of 5G networks, (d) normalized energy consumption of 5G networks. After years of optimization of 4G base station deployments, the energy consumption of 4G, related to the number of base stations, is with a similar spatial distribution of the traffic loads. In contrast, due to the lack of traffic profiles of 5G applications, the deployment of 5G base stations is not optimized. The spatial distribution of 5G network traffic load and energy consumption shows big differences. . . . . . . . . . . . . . . . . . 15
S4 Performance of DeepEnergy on 4G and 5G networks. (a). Temporal distribution of misalignment factors of the 4G networks in Nanchang. (b). Spatial distribution of misalignment factor of the 4G networks in Nanchang. (c). Temporal distribution of misalignment factors of the 5G networks in Nanchang. (d). Spatial distribution of misalignment factors of the 5G networks in Nanchang. DeepEnergy significantly reduces the misalignment between energy consumption and cellular traffic in both 4G and 5G networks. . . . . . . . . . . . . . . . . . . . . . . . . . . . . . . . . . 16
S5 The distribution of the grid emission factors derived from the proposed simulation-based model based on Nanchang's data. There is no significant difference in grid emission factors before and after launching the 5G network. . . . . . . . . . . . . . 17
S6 The energy-traffic curve for mobile networks in Nanchang. Network energy is not proportional to the amount of network traffic it carries (see red dots). The green dashed line represents the desired energy, which is proportional to the volume of traffic. The green star point denotes the $(C, E_{Max})$ point, where $C$ represents network capacity, which is the maximum amount of traffic that the mobile network can support, and $E_{Max}$ represents the corresponding amount of energy consumed. 18
S7 A typical base station in mobile networks. A base station consists of a communication subsystem and a supporting subsystem. The communication subsystem includes the Remote Radio Unit (RRU) and Base Band Unit (BBU), while the supporting subsystem includes the cooling and other auxiliary devices. . . . . . . 19
S8 BBU power of a base station is related to the number of cells it has. Generally, base stations with more cells have more BBUs. The BBU power of a particular BS type is mainly distributed in a small interval. . . . . . . . . . . . . . . . . . . . . . . . . 20
S9 In 5G networks, RRU power ($P_{RRU}$) and transmit power ($P_{trans}$) show a strong linear relationship. Different base station types have specific settings of maximum transmit power. '32TR' and '64TR' denote the number of base station antennas. 'NSA' and 'SA' refer to non-standalone architecture and standalone architecture, respectively. . . . . . . . . . . . . . . . . . . . . . . . . . . . . . . . . . . . . . . . 21
S10 Linear models can approximate the relationships between RRU power ($P_{RRU}$) and transmit power ($P_{trans}$) for a variety of 5G base stations with high accuracy. . . . . 22
S11 Scatter plot of RRU power and transmit power for 4G base stations. Linear models can approximate the relationships between RRU power ($P_{RRU}$) and transmit power ($P_{trans}$) for a variety of 4G base stations with a high accuracy. . . . . . . . . . . . . . 23
S12 Scatter plot of transmit power and PRB usage ratio in 5G networks. Transmit power and PRB usage ratio have a significant linear relationship. . . . . . . . . . . 24
S13 Linear models can approximate the relationships between transmit power ($P_{trans}$) and PRB usage ratio $r_{PRB}$ for a variety of 5G base stations with a high accuracy. . . 25
S14 (a) Scatter plot of transmit power and PRB usage ratio in 4G networks. Significant linear correlation exists between transmit power and PRB usage ratio. (b)-(d) Linear models can accurately approximate the relationships between transmit power and traffic load (i.e., PRB usage ratio) for various 4G base stations. The slopes and offsets of the regression model vary depending on the base station settings. . . . . 26
S15 The cumulative distribution function (CDF) of RRU power in sleep mode. a) 4G base stations. b) 5G base stations. . . . . . . . . . . . . . . . . . . . . . . . . . . . . . . 27

S16 Typical load curve in Jiangxi province: (a) load curve of a year; (b) load curve in a working day; (c) load curve in a weekend day. . . . . . . . . . . . . . . . . . . . . . . 28
S17 Comparison of the static approximation and dynamic approximation method to compute $P_{orig}(t)$: (a) carbon emissions caused by 4G BS power load from 20 May to 26 May; (b) carbon emissions caused by 5G base station power load from 20 May to 26 May; (c) $P_{orig}(t)$ computed by the dynamic approximation method from 20 May to 26 May, and the resulted power generation of XinChang unit 1 and 2 during 23 May and 24 May; (d) extra power generation of XinChang unit 1 and 2 specifically for 4G and 5G base station load during 23 May and 24 May. . . . . . . 29
S18 When the PRB usage ratio (or traffic load) of base station A is low, base station A enters sleep mode and the mobile user served is offloaded to adjacent base station B. In this case, base station B is the compensating base station of base station A. . . 30
S19 The neural network architecture of the action-value network. The information of the cells from the same grid or the same base station are integrate to predict the rewards for different actions. . . . . . . . . . . . . . . . . . . . . . . . . . . . . . . 31
S20 Misalignment factor vs. the normalized network traffic load for various Energy-saving scenarios. Under a specific Energy-saving scenario, the misalignment factor ($M$) linearly decreases as the normalized network traffic load ($\tilde{L}$) increases. . . . . . 32
S21 Linear models can approximate the relationships between the normalized network traffic load ($\tilde{L}$) and the misalignment factor ($M$) with high accuracy. . . . . . . . . . 33
S22 We partition Nanchang into four regions, according to the city center point, and denote them as Region A, Region B, Region C, and Region D. These four regions have different base station densities, network capacities, and network traffic loads. 34
S23 For DeepEnergy models trained on different regions, Linear models can approximate the relationships between the normalized network traffic load ($\tilde{L}$) and the misalignment factor ($M$) with high accuracy. . . . . . . . . . . . . . . . . . . . . . . 35

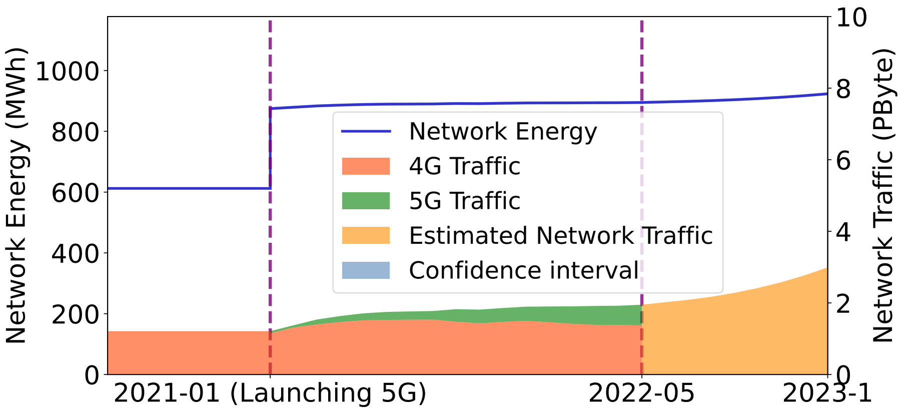


(a)

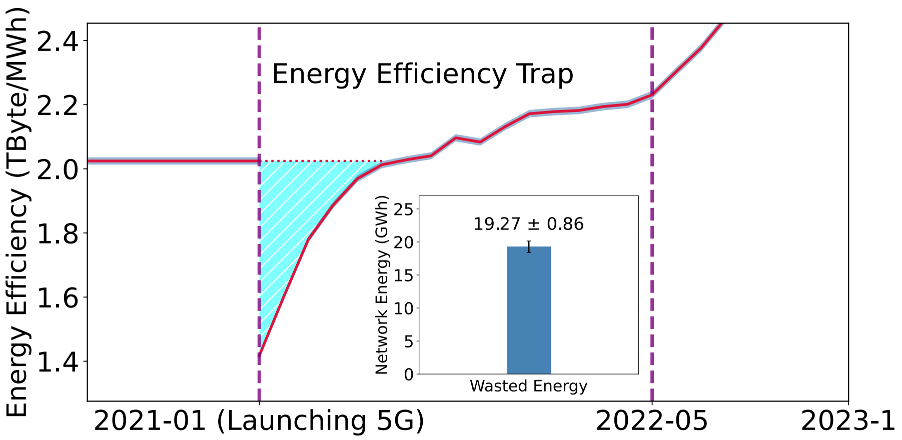


(b)

**Fig. S1.** Launching 5G Leads to the appearance of energy efficiency trap in Nanchang. (a) The operation of newly launched 5G base stations has led to a sharp increase in energy consumption in Nanchang. (c) Launching 5G Leads to the appearance of an energy efficiency trap and causes extra energy consumption in Nanchang.

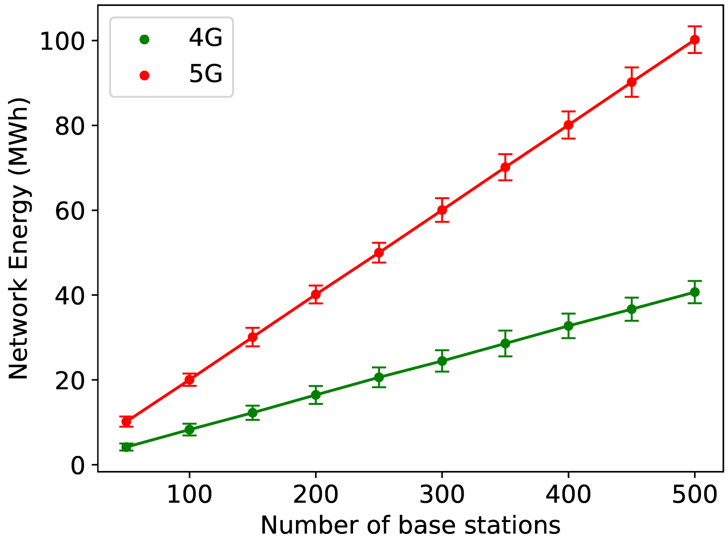


**Fig. S2.** The daily energy consumption vs. the number of base stations. The energy consumption of a mobile network are highly correlated with its number of base stations.

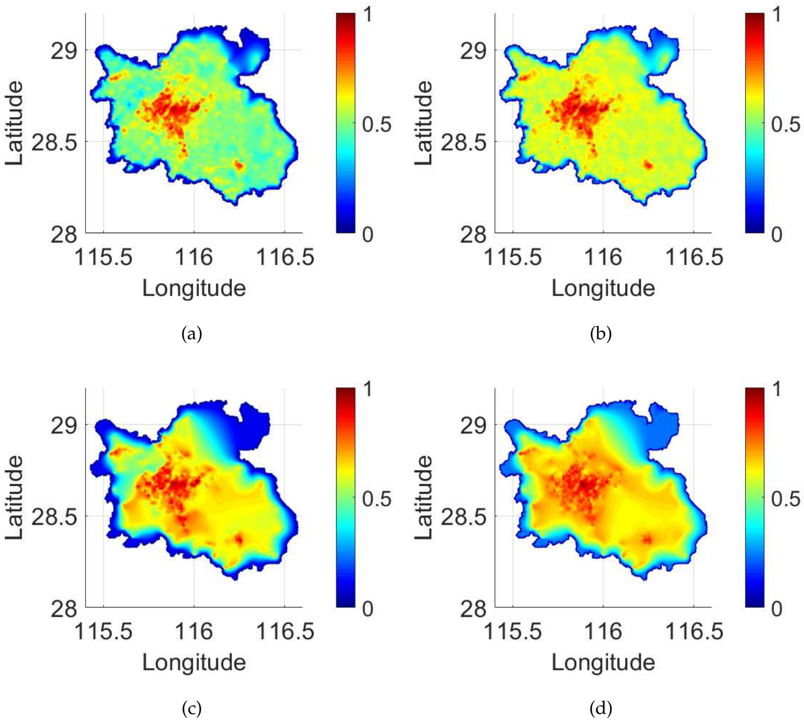


**Fig. S3.** The spatial distribution of (a) normalized traffic loads of 4G networks, (b) normalized energy consumption of 4G networks, (c) normalized traffic loads of 5G networks, (d) normalized energy consumption of 5G networks. After years of optimization of 4G base station deployments, the energy consumption of 4G, related to the number of base stations, is with a similar spatial distribution of the traffic loads. In contrast, due to the lack of traffic profiles of 5G applications, the deployment of 5G base stations is not optimized. The spatial distribution of 5G network traffic load and energy consumption shows big differences.

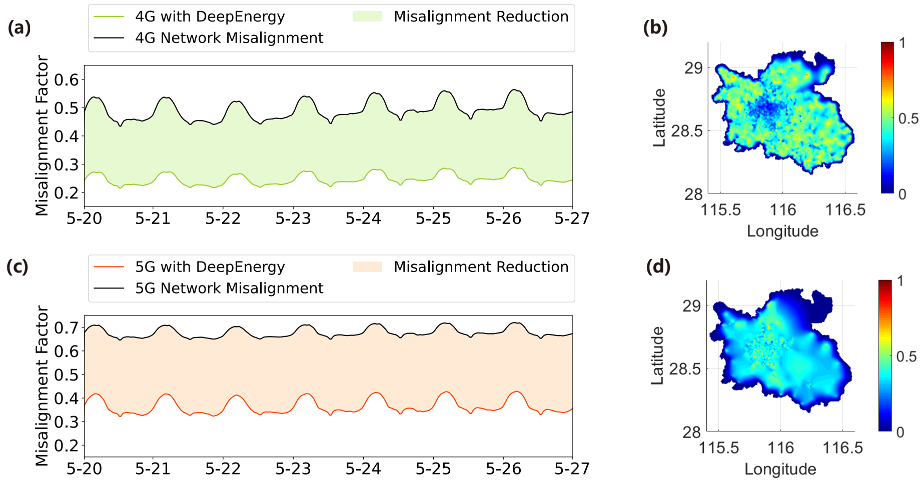


**Fig. S4.** Performance of DeepEnergy on 4G and 5G networks. (a). Temporal distribution of misalignment factors of the 4G networks in Nanchang. (b). Spatial distribution of misalignment factor of the 4G networks in Nanchang. (c). Temporal distribution of misalignment factors of the 5G networks in Nanchang. (d). Spatial distribution of misalignment factors of the 5G networks in Nanchang. DeepEnergy significantly reduces the misalignment between energy consumption and cellular traffic in both 4G and 5G networks.

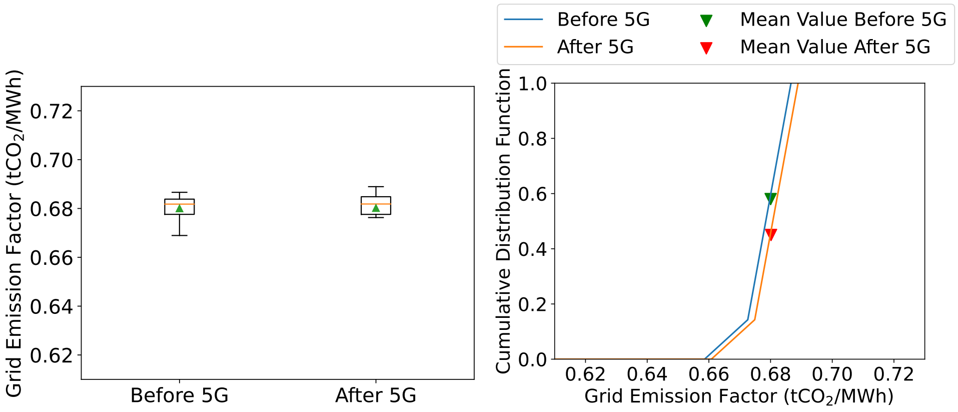


(a) The box-plot of grid emission factors.

(b) The cumulative distribution function (CDF) of grid emission factors.

**Fig. S5.** The distribution of the grid emission factors derived from the proposed simulation-based model based on Nanchang's data. There is no significant difference in grid emission factors before and after launching the 5G network.

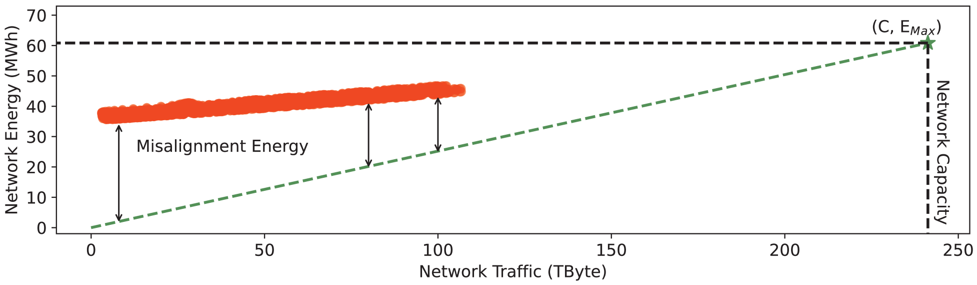


**Fig. S6.** The energy-traffic curve for mobile networks in Nanchang. Network energy is not proportional to the amount of network traffic it carries (see red dots). The green dashed line represents the desired energy, which is proportional to the volume of traffic. The green star point denotes the $(C, E_{Max})$ point, where $C$ represents network capacity, which is the maximum amount of traffic that the mobile network can support, and $E_{Max}$ represents the corresponding amount of energy consumed.

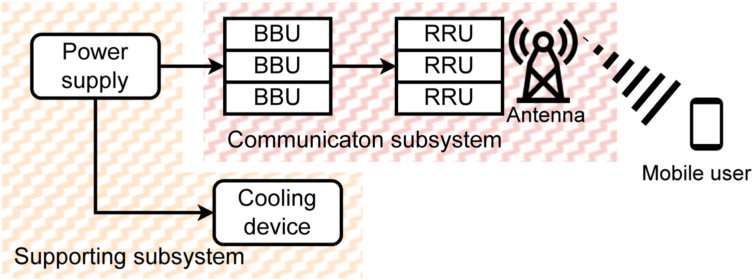


**Fig. S7.** A typical base station in mobile networks. A base station consists of a communication subsystem and a supporting subsystem. The communication subsystem includes the Remote Radio Unit (RRU) and Base Band Unit (BBU), while the supporting subsystem includes the cooling and other auxiliary devices.

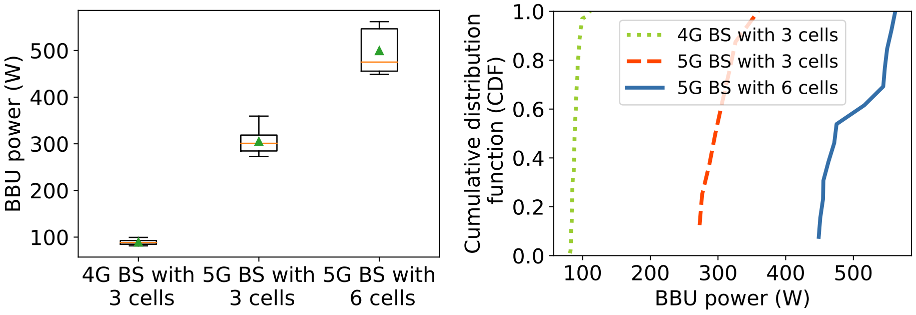


(a) The box-plot of BBU power.

(b) The cumulative distribution function (CDF) of BBU power.

**Fig. S8.** BBU power of a base station is related to the number of cells it has. Generally, base stations with more cells have more BBUs. The BBU power of a particular BS type is mainly distributed in a small interval.

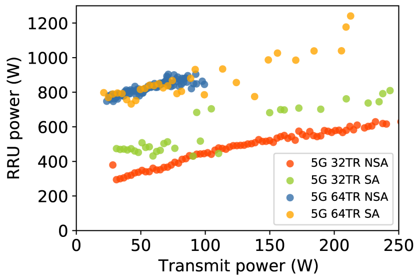


(a) Scatter plot of RRU power and transmit power in 5G networks.

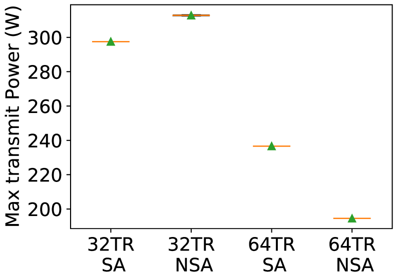


(b) Maximum transmit power distribution of different 5G base station types.

**Fig. S9.** In 5G networks, RRU power ($P_{RRU}$) and transmit power ($P_{trans}$) show a strong linear relationship. Different base station types have specific settings of maximum transmit power. '32TR' and '64TR' denote the number of base station antennas. 'NSA' and 'SA' refer to non-standalone architecture and standalone architecture, respectively.

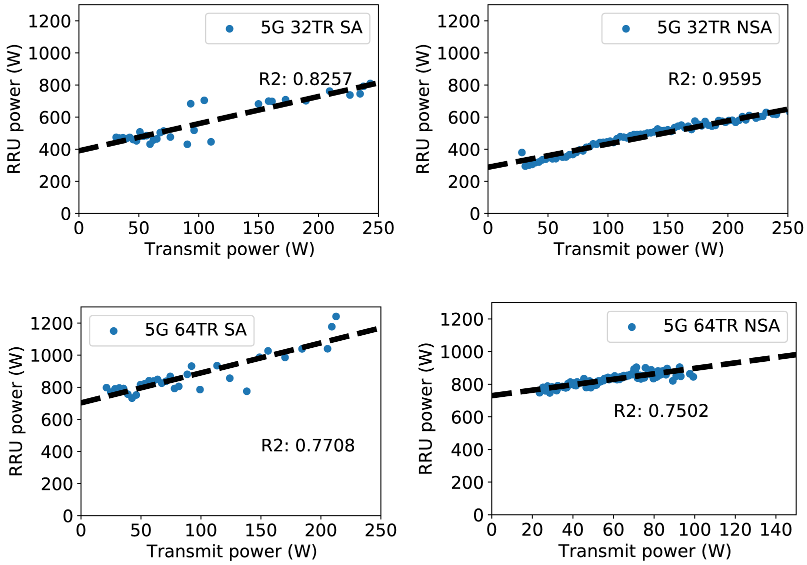


**Fig. S10.** Linear models can approximate the relationships between RRU power ($P_{RRU}$) and transmit power ($P_{trans}$) for a variety of 5G base stations with high accuracy.

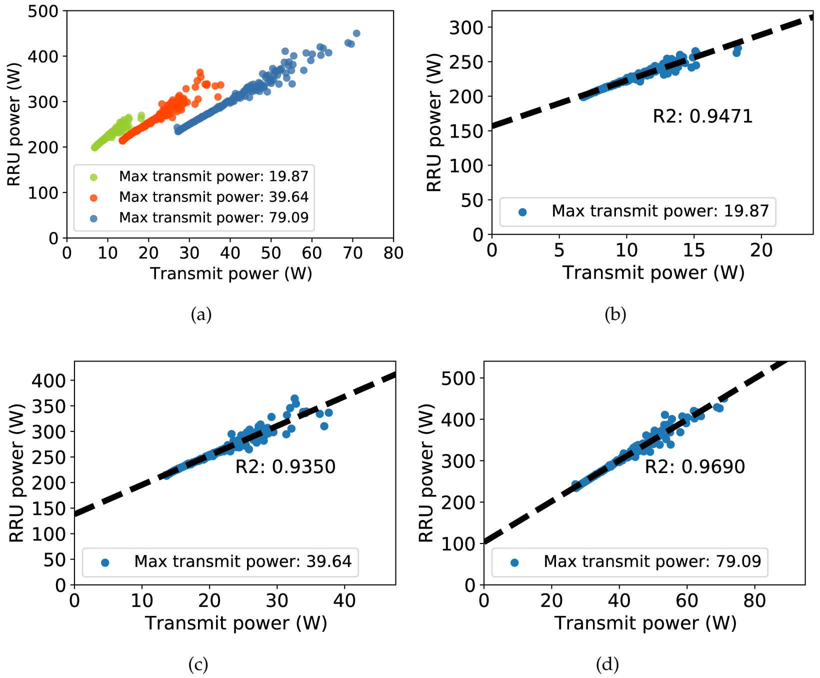


**Fig. S11.** Scatter plot of RRU power and transmit power for 4G base stations. Linear models can approximate the relationships between RRU power ($P_{RRU}$) and transmit power ($P_{trans}$) for a variety of 4G base stations with a high accuracy.

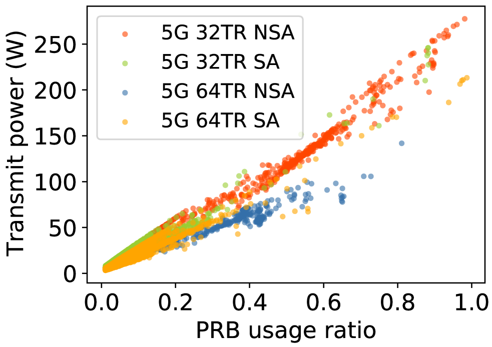


**Fig. S12.** Scatter plot of transmit power and PRB usage ratio in 5G networks. Transmit power and PRB usage ratio have a significant linear relationship.

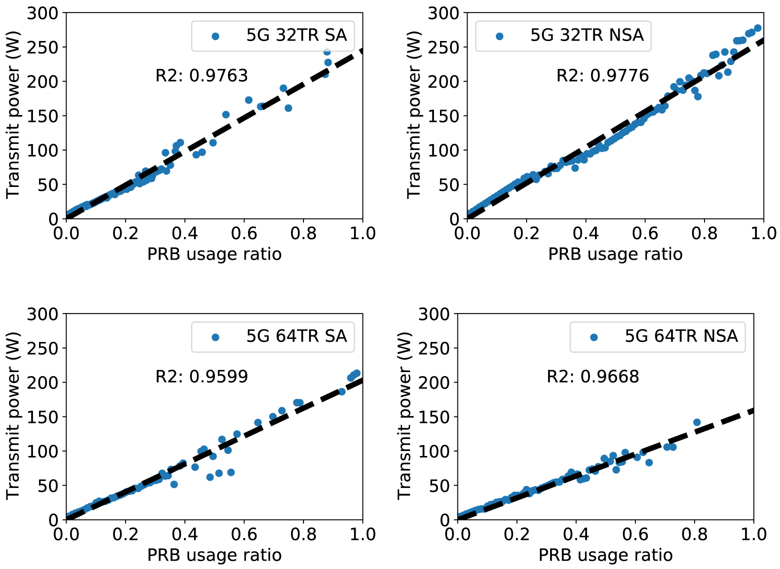


**Fig. S13.** Linear models can approximate the relationships between transmit power $(P_{trans})$ and PRB usage ratio $r_{PRB}$ for a variety of 5G base stations with a high accuracy.

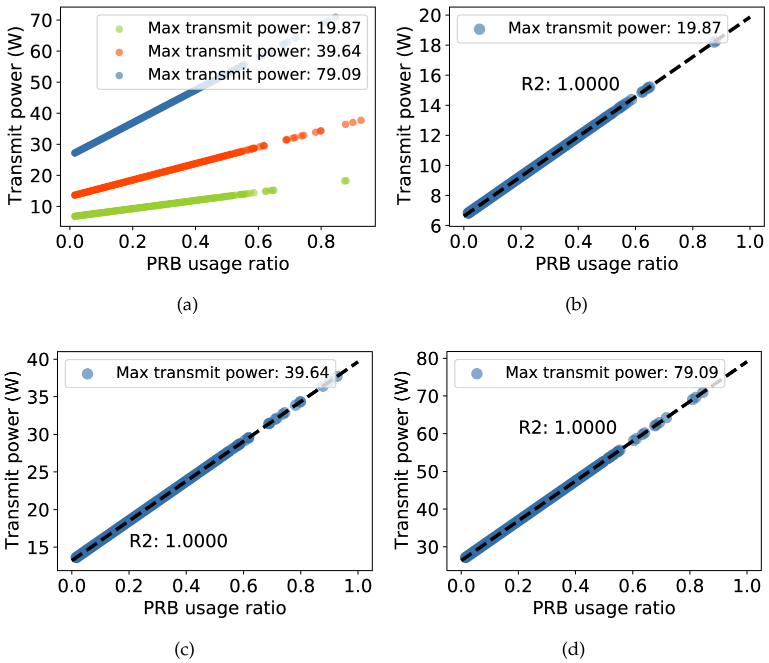


**Fig. S14.** (a) Scatter plot of transmit power and PRB usage ratio in 4G networks. Significant linear correlation exists between transmit power and PRB usage ratio. (b)-(d) Linear models can accurately approximate the relationships between transmit power and traffic load (i.e., PRB usage ratio) for various 4G base stations. The slopes and offsets of the regression model vary depending on the base station settings.

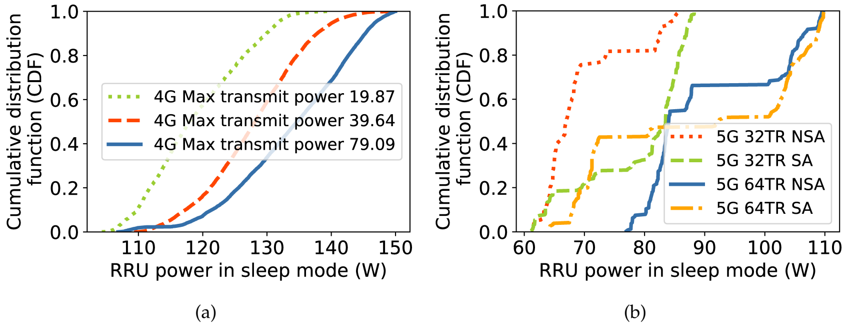


**Fig. S15.** The cumulative distribution function (CDF) of RRU power in sleep mode. a) 4G base stations. b) 5G base stations.

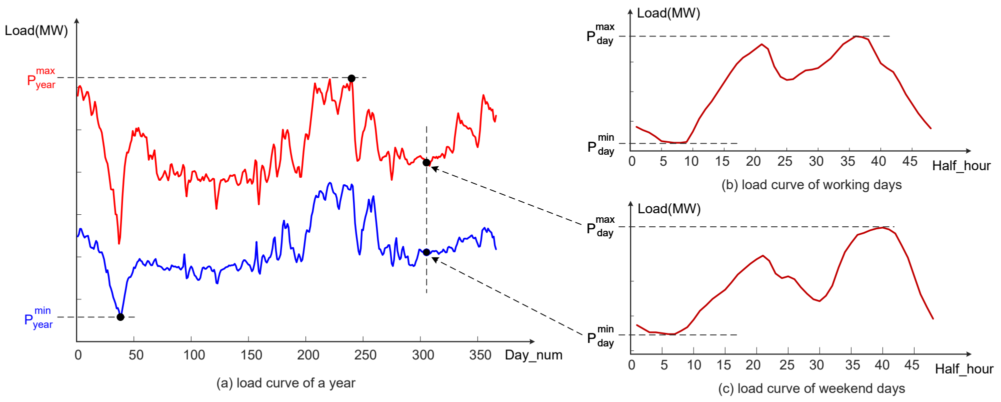


**Fig. S16.** Typical load curve in Jiangxi province: (a) load curve of a year; (b) load curve in a working day; (c) load curve in a weekend day.

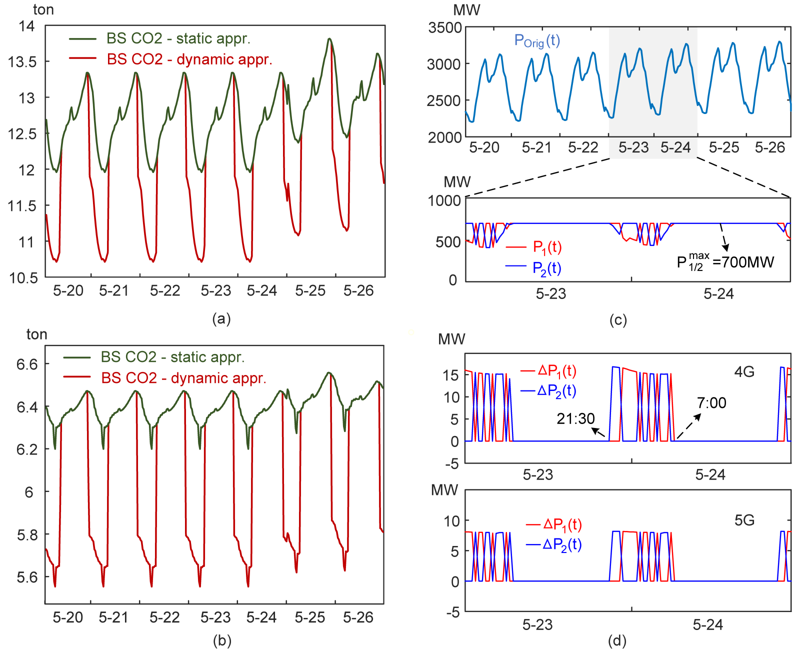


**Fig. S17.** Comparison of the static approximation and dynamic approximation method to compute $P_{orig}(t)$: (a) carbon emissions caused by 4G BS power load from 20 May to 26 May; (b) carbon emissions caused by 5G base station power load from 20 May to 26 May; (c) $P_{orig}(t)$ computed by the dynamic approximation method from 20 May to 26 May, and the resulted power generation of XinChang unit 1 and 2 during 23 May and 24 May; (d) extra power generation of XinChang unit 1 and 2 specifically for 4G and 5G base station load during 23 May and 24 May.

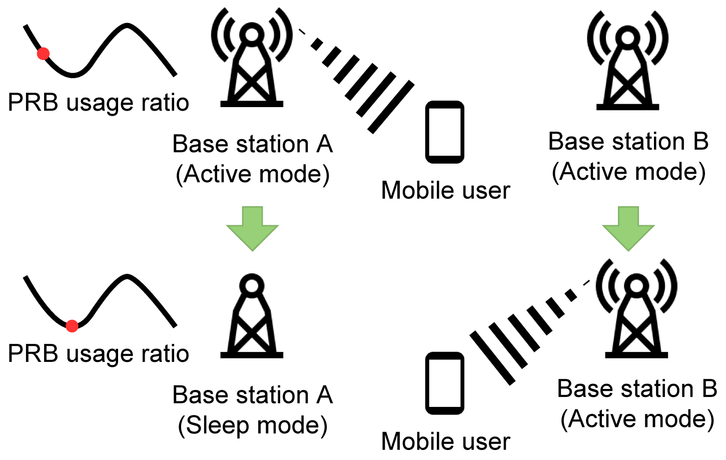


**Fig. S18.** When the PRB usage ratio (or traffic load) of base station A is low, base station A enters sleep mode and the mobile user served is offloaded to adjacent base station B. In this case, base station B is the compensating base station of base station A.

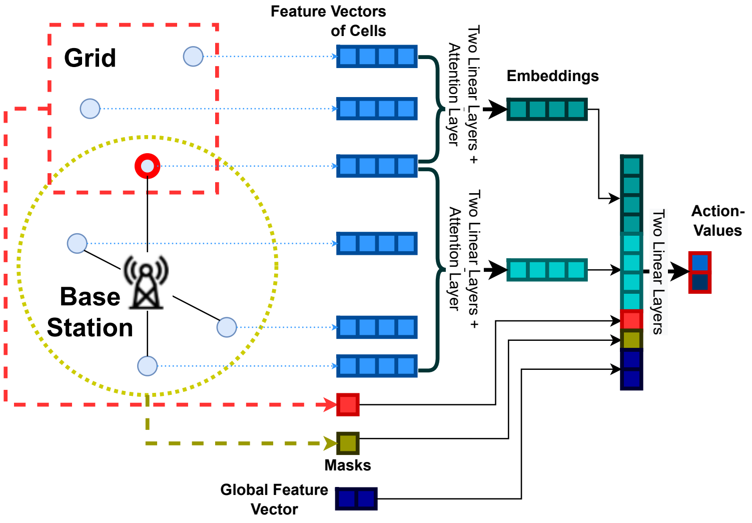


**Fig. S19.** The neural network architecture of the action-value network. The information of the cells from the same grid or the same base station are integrate to predict the rewards for different actions.

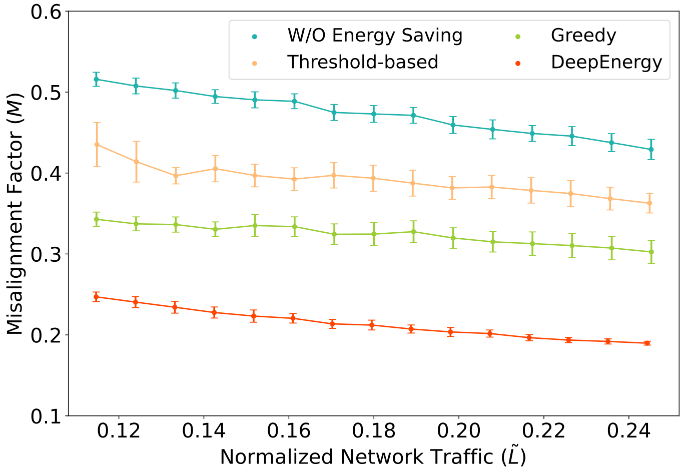


**Fig. S20.** Misalignment factor vs. the normalized network traffic load for various Energy-saving scenarios. Under a specific Energy-saving scenario, the misalignment factor ($M$) linearly decreases as the normalized network traffic load ($\tilde{L}$) increases.

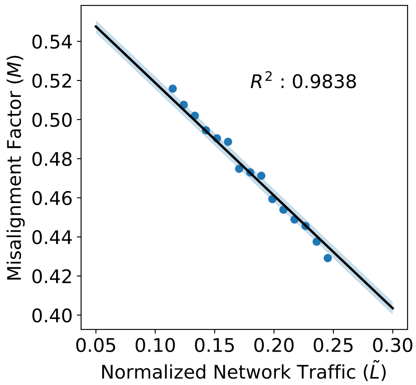


(a) Without energy-saving

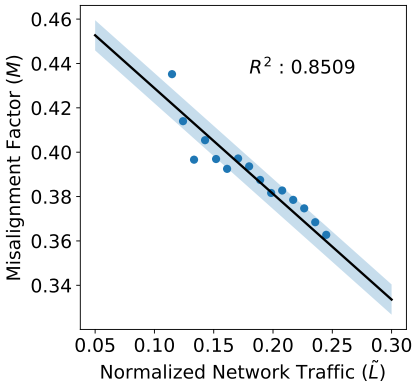


(b) Threshold-based energy-saving Method

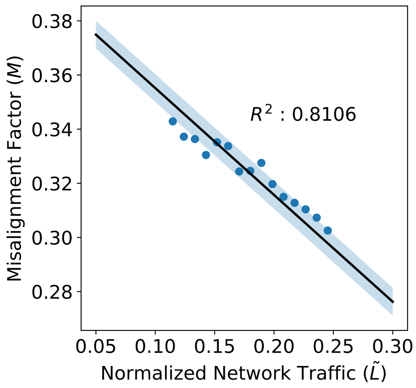


(c) Greedy energy-saving Method

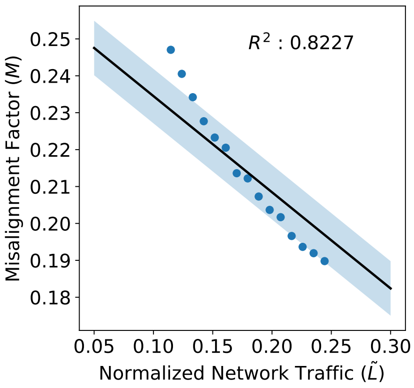


(d) DeepEnergy

**Fig. S21.** Linear models can approximate the relationships between the normalized network traffic load ($\tilde{L}$) and the misalignment factor ($M$) with high accuracy.

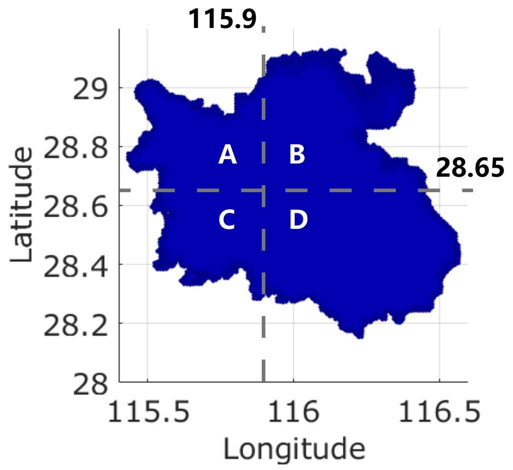


**Fig. S22.** We partition Nanchang into four regions, according to the city center point, and denote them as Region A, Region B, Region C, and Region D. These four regions have different base station densities, network capacities, and network traffic loads.

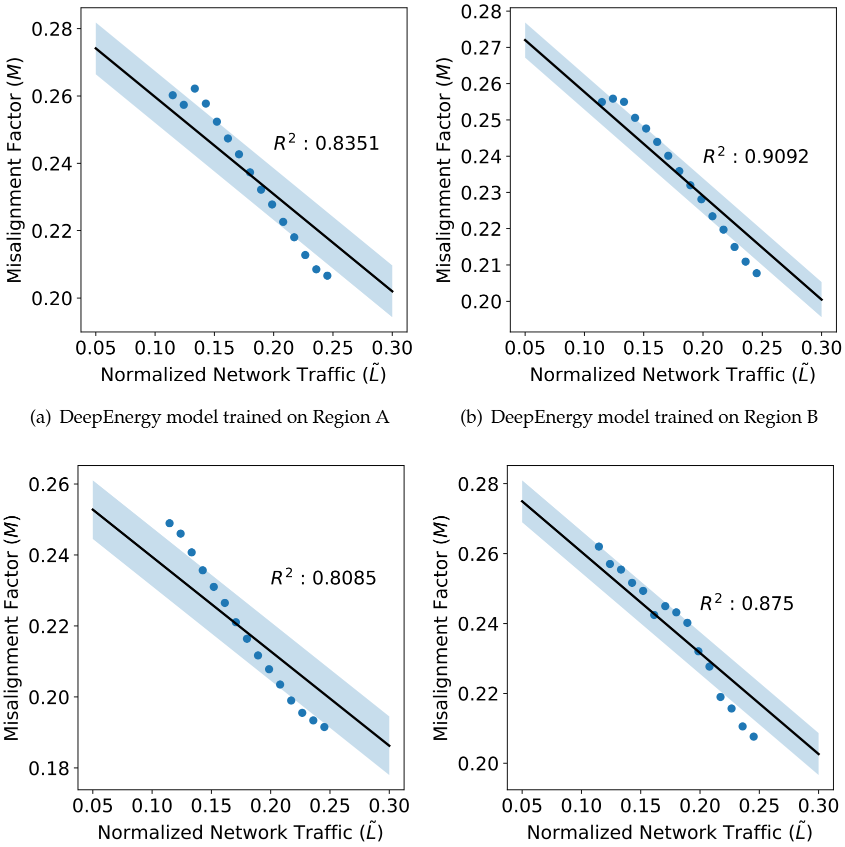


(a) DeepEnergy model trained on Region A

(b) DeepEnergy model trained on Region B

(c) DeepEnergy model trained on Region C

(d) DeepEnergy model trained on Region D

**Fig. S23.** For DeepEnergy models trained on different regions, Linear models can approximate the relationships between the normalized network traffic load ($\tilde{L}$) and the misalignment factor ($M$) with high accuracy.

## LIST OF TABLES

S1 The collected data items of energy consumption data and network traffic data. (NA refers to 'not available'.) . . . 37
S2 Monthly network traffic statistics in Nanchang, measured in PBytes. And, the number of mobile users in Nanchang, expressed as a million. . . . 38
S3 The number of 4G and 5G base stations across different provinces in China as of January 2021. . . . 39
S4 The number of mobile users across China's various provinces, expressed as a million. 40
S5 Parameter setting of PV system simulation . . . 41
S6 Generation unit configuration in Nanchang. . . . 42
S7 Additional carbon emissions across different provinces in China, the unit is $KtCO_2$. 43
S8 Wasted energy consumption across different provinces in China, the unit is GWh. . 44
S9 Reduction in carbon emissions using different energy-saving methods across different provinces in China in 2021 compared to the case without energy-saving, the unit is $KtCO_2$. . . . 45
S10 Reduction in carbon emissions using different energy-saving methods across different provinces in China in 2022 compared to the case without energy-saving, the unit is $KtCO_2$. . . . 46
S11 Reduction in carbon emissions using different energy-saving methods across different provinces in China in 2023 compared to the case without energy-saving, the unit is $KtCO_2$. . . . 47
S12 Reduction in energy consumption using different energy-saving methods across different provinces in China in 2021 compared to the case without energy-saving, the unit is GWh. . . . 48
S13 Reduction in energy consumption using different energy-saving methods across different provinces in China in 2022 compared to the case without energy-saving, the unit is MWh. . . . 49
S14 Reduction in energy consumption using different energy-saving methods across different provinces in China in 2023 compared to the case without energy-saving, the unit is GWh. . . . 50
S15 Energy consumption of mobile networks across different province in China over years, the unit is GWh. . . . 51
S16 Carbon emissions of mobile networks across different province in China over years, the unit is $KtCO_2$. . . . 52
S17 Data used for investment, operation and maintenance costs of photovoltaic system. 53
S18 Number of base stations and $R^2$ score of estimated $M$ and ground truth in four regions. . . . 54
S19 The $R^2$ score of estimated $M$ and ground truth of different traffic load. . . . 55
S20 Average and standard deviation of BBU power for different types of base stations. 56
S21 Linear regression analysis for RRU power consumption in 5G networks. . . . 57
S22 Linear regression analysis for RRU power consumption in 4G networks. . . . 58
S23 Average and standard deviation of RRU power in sleep mode for different types of base stations. . . . 59
S24 Parameter settings of EnergyPlus to simulation the power consumption of base stations' cooling subsystem. . . . 60
S25 Parameter settings of the threshold-based method used in current real-world mobile networks. (NA refers to 'not available') . . . 61
S26 Linear regression analysis for misalignment factor. . . . 62
S27 The estimated misalignment factors across provinces without energy-saving. . . . 63
S28 The estimated misalignment factors across provinces with threshold-based energy-saving method. . . . 64
S29 The estimated misalignment factors across provinces with greedy energy-saving method. . . . 65
S30 The estimated misalignment factors across provinces with DeepEnergy. . . . 66
S31 The performance of the models trained on data from different regions in Nanchang. 67
S32 Linear regression analysis for misalignment factor of DeepEnergy models trained on different regions. . . . 68

**Table S1.** The collected data items of energy consumption data and network traffic data. (NA refers to 'not available'.)

| Items collected | Description | Power consumption data | Network performance data |
|---|---|---|---|
| Base station ID | An unique identification for the base station where the data is collected | √ | √ |
| Timestamp | The time the record was gathered | √ | √ |
| PRB usage ratio | The percentage of the base station's total available physical resource blocks (PRB) that are currently being utilized | √ | √ |
| Traffic volume | Average volume of downlink traffic, measured in KBytes | √ | √ |
| # of users | Average number of users served | √ | √ |
| Data rate | Average downlink data rate of users served, measured in Mbps | √ | √ |
| Transmit power | Average transmit power of the base station, measured in Watts | √ | NA |
| BBU power | Average power consumption of the base station's base band units (BBU), measured in Watts | √ | NA |
| RRU power | Average power consumption of the base station's remote radio units (RRU), measured in Watts | √ | NA |
| Element power | Average power consumption of the base station, measured in Watts | √ | NA |
| Sleep time | Average time of the base station is in sleep mode | √ | NA |

**Table S2.** Monthly network traffic statistics in Nanchang, measured in PBytes. And, the number of mobile users in Nanchang, expressed as a million.

| Month | Traffic volume of 4G networks | Traffic volume of 5G networks | Traffic volume of mobile networks | Number of mobile users |
|---|---|---|---|---|
| 2021-01 | 1.1536 | 0.0569 | 1.2105 | 7.241 |
| 2021-02 | 1.3128 | 0.0622 | 1.375 | 7.218 |
| 2021-03 | 1.3991 | 0.1364 | 1.5355 | 7.344 |
| 2021-04 | 1.4649 | 0.1673 | 1.6322 | 7.386 |
| 2021-05 | 1.5131 | 0.1953 | 1.7084 | 7.433 |
| 2021-06 | 1.5246 | 0.2237 | 1.7483 | 7.524 |
| 2021-07 | 1.5306 | 0.2319 | 1.7625 | 7.575 |
| 2021-08 | 1.5333 | 0.2405 | 1.7738 | 7.626 |
| 2021-09 | 1.4736 | 0.3518 | 1.8254 | 7.797 |
| 2021-10 | 1.4311 | 0.3821 | 1.8132 | 7.816 |
| 2021-11 | 1.4701 | 0.3870 | 1.8571 | 7.827 |
| 2021-12 | 1.4985 | 0.3963 | 1.8948 | 7.838 |
| 2022-01 | 1.4614 | 0.4394 | 1.9008 | 7.981 |
| 2022-02 | 1.4159 | 0.4881 | 1.9040 | 8.048 |
| 2022-03 | 1.3873 | 0.5280 | 1.9153 | 8.084 |
| 2022-04 | 1.3820 | 0.5400 | 1.9220 | 7.960 |
| 2022-05 | 1.3719 | 0.5777 | 1.9496 | 7.874 |

**Table S3.** The number of 4G and 5G base stations across different provinces in China as of January 2021.

| Province | # of 4G Base Stations | # of 5G Base Stations |
|---|---|---|
| Beijing | 24305 | 15293 |
| Tianjing | 15009 | 9451 |
| Hebei | 107949 | 38758 |
| Shanxi | 64850 | 26122 |
| Inner Mongolia | 36502 | 15993 |
| Liaoning | 63647 | 19745 |
| Jilin | 32089 | 9590 |
| Heilongjiang | 46940 | 21158 |
| Shanghai | 25672 | 24881 |
| Jiangsu | 93128 | 69458 |
| Zhejiang | 92217 | 58079 |
| Anhui | 71780 | 35477 |
| Fujian | 96086 | 29828 |
| Jiangxi | 71101 | 37764 |
| Shandong | 117311 | 58687 |
| Henan | 97658 | 34639 |
| Hubei | 82828 | 37536 |
| Hunan | 84584 | 31804 |
| Guangdong | 124663 | 90689 |
| Guangxi | 72839 | 20929 |
| Hainan | 14808 | 6690 |
| Chongqing | 60704 | 23969 |
| Sichuan | 149584 | 35068 |
| Guizhou | 79910 | 33592 |
| Yunnan | 106092 | 42795 |
| Tibet | 16502 | 2880 |
| Shaanxi | 61301 | 24552 |
| Gansu | 48530 | 10034 |
| Qinghai | 12547 | 3246 |
| Ningxia | 11556 | 5588 |
| Xinjiang | 48386 | 10964 |

**Table S4.** The number of mobile users across China's various provinces, expressed as a million.

| Province | 2021-01 | 2021-02 | 2021-03 | 2021-04 | 2021-05 | 2021-06 | 2021-07 | 2021-08 | 2021-09 | 2021-10 | 2021-11 | 2021-12 | 2022-01 | 2022-02 | 2022-03 | 2022-04 | 2022-05 |
|---|---|---|---|---|---|---|---|---|---|---|---|---|---|---|---|---|---|
| Beijing | 39.064 | 38.704 | 38.643 | 38.51 | 38.461 | 38.661 | 38.835 | 39.178 | 39.458 | 39.32 | 39.464 | 39.72 | 39.5035 | 39.287 | 39.338 | 39.398 | 39.407 |
| Tianjing | 17.11 | 17.064 | 17.136 | 17.187 | 17.194 | 17.363 | 17.361 | 17.244 | 17.29 | 17.421 | 17.448 | 17.451 | 17.439 | 17.427 | 17.484 | 17.531 | 17.415 |
| Hebei | 83.36 | 83.477 | 83.912 | 84.032 | 84.061 | 84.304 | 84.699 | 85.064 | 85.718 | 86.015 | 86.106 | 86.435 | 86.5345 | 86.634 | 86.613 | 86.512 | 86.479 |
| Shanxi | 40.228 | 40.182 | 40.45 | 40.402 | 40.394 | 40.67 | 40.681 | 40.822 | 41.141 | 41.154 | 41.137 | 41.26 | 41.308 | 41.356 | 41.677 | 41.626 | 41.725 |
| Inner Mongolia | 29.622 | 29.457 | 29.567 | 29.505 | 29.489 | 29.482 | 29.537 | 29.663 | 29.76 | 29.802 | 29.972 | 30.169 | 30.1345 | 30.10 | 30.245 | 30.274 | 30.335 |
| Liaoning | 48.738 | 48.579 | 48.848 | 48.864 | 48.884 | 48.965 | 49.061 | 49.191 | 49.681 | 49.719 | 49.720 | 49.752 | 49.73 | 49.708 | 50.068 | 49.941 | 50.102 |
| Jilin | 28.701 | 28.571 | 28.765 | 28.77 | 28.884 | 29.01 | 29.104 | 29.153 | 29.324 | 29.376 | 29.563 | 29.665 | 29.6765 | 29.688 | 29.597 | 29.415 | 29.674 |
| Heilongjiang | 38.444 | 37.258 | 37.397 | 37.314 | 37.423 | 37.455 | 37.395 | 37.437 | 37.827 | 38.007 | 38.129 | 37.595 | 37.7335 | 37.872 | 37.926 | 37.995 | 38.078 |
| Shanghai | 42.776 | 42.729 | 42.938 | 43.389 | 43.78 | 43.969 | 44.159 | 44.314 | 44.459 | 44.591 | 44.714 | 43.988 | 44.016 | 44.044 | 44.019 | 43.592 | 42.854 |
| Jiangsu | 98.971 | 99.075 | 99.671 | 99.586 | 99.767 | 100.184 | 100.412 | 100.508 | 100.814 | 101.449 | 101.579 | 101.795 | 102.254 | 102.713 | 103.358 | 103.302 | 103.628 |
| Zhejiang | 85.852 | 85.102 | 85.643 | 86.473 | 86.796 | 87.018 | 87.432 | 87.978 | 88.425 | 88.628 | 88.625 | 88.596 | 88.833 | 89.07 | 89.93 | 90.098 | 90.45 |
| Anhui | 60.256 | 60.558 | 60.762 | 60.932 | 61.312 | 61.532 | 61.648 | 61.835 | 62.028 | 62.069 | 62.027 | 61.926 | 62.2785 | 62.631 | 62.856 | 62.846 | 62.911 |
| Fujian | 47.393 | 47.275 | 47.603 | 47.708 | 47.813 | 47.912 | 47.859 | 48.204 | 48.395 | 48.475 | 48.485 | 48.243 | 48.3355 | 48.428 | 48.633 | 48.614 | 48.604 |
| Jiangxi | 42.494 | 43.007 | 43.323 | 43.399 | 43.617 | 44.007 | 44.187 | 44.574 | 44.978 | 45.139 | 44.769 | 44.968 | 45.6215 | 46.275 | 46.421 | 45.896 | 44.94 |
| Shandong | 109.071 | 108.654 | 109.231 | 109.601 | 109.944 | 110.074 | 110.492 | 110.994 | 111.506 | 112.203 | 112.214 | 112.485 | 112.931 | 113.377 | 114.236 | 114.586 | 115.179 |
| Henan | 100.514 | 101.16 | 101.813 | 101.833 | 101.949 | 102.311 | 102.50 | 102.459 | 102.783 | 103.426 | 103.421 | 103.526 | 103.7915 | 104.057 | 104.478 | 104.558 | 104.641 |
| Hubei | 56.811 | 57.061 | 57.48 | 57.45 | 57.514 | 57.661 | 57.726 | 58.264 | 58.637 | 58.868 | 58.935 | 58.711 | 58.862 | 59.013 | 59.254 | 59.381 | 59.411 |
| Hunan | 67.194 | 67.612 | 67.859 | 68.002 | 68.367 | 68.538 | 68.894 | 68.954 | 69.519 | 69.521 | 69.387 | 69.423 | 69.347 | 69.271 | 69.43 | 69.405 | 69.521 |
| Guangdong | 155.369 | 153.943 | 154.715 | 156.70 | 157.088 | 157.586 | 158.84 | 159.857 | 161.224 | 162.058 | 162.541 | 162.678 | 162.8955 | 163.113 | 165.621 | 166.343 | 166.69 |
| Guangxi | 53.329 | 53.796 | 54.061 | 54.012 | 54.018 | 54.008 | 54.288 | 54.716 | 54.971 | 55.125 | 55.077 | 55.114 | 55.233 | 55.352 | 56.063 | 56.231 | 56.616 |
| Hainan | 11.352 | 11.195 | 11.374 | 11.366 | 11.368 | 11.324 | 11.298 | 11.285 | 11.502 | 11.566 | 11.573 | 11.589 | 11.564 | 11.539 | 11.734 | 11.633 | 11.571 |
| Chongqing | 36.401 | 36.691 | 36.92 | 36.849 | 36.906 | 36.928 | 37.031 | 37.284 | 37.571 | 37.663 | 37.612 | 37.511 | 37.8435 | 38.176 | 38.356 | 38.408 | 38.509 |
| Sichuan | 91.246 | 91.53 | 91.995 | 91.473 | 91.695 | 92.587 | 92.677 | 92.692 | 92.894 | 93.117 | 93.154 | 93.389 | 93.7805 | 94.172 | 94.835 | 95.082 | 95.168 |
| Guizhou | 40.935 | 41.162 | 41.483 | 41.363 | 41.382 | 41.409 | 41.448 | 42.026 | 42.228 | 42.404 | 42.436 | 42.699 | 42.871 | 43.043 | 43.292 | 43.27 | 43.312 |
| Yunnan | 49.534 | 49.706 | 50.103 | 49.95 | 49.623 | 49.715 | 50.02 | 50.271 | 50.473 | 50.321 | 50.359 | 50.457 | 50.4385 | 50.42 | 50.63 | 50.583 | 50.478 |
| Tibet | 3.219 | 3.155 | 3.138 | 3.197 | 3.195 | 3.212 | 3.245 | 3.258 | 3.305 | 3.322 | 3.316 | 3.334 | 3.3235 | 3.313 | 3.344 | 3.355 | 3.349 |
| Shaanxi | 45.897 | 45.534 | 45.405 | 46.095 | 46.222 | 46.735 | 47.069 | 47.242 | 47.496 | 47.681 | 47.720 | 47.778 | 47.728 | 47.678 | 48.373 | 47.964 | 48.045 |
| Gansu | 26.738 | 26.69 | 26.912 | 26.937 | 27.069 | 27.178 | 27.221 | 27.308 | 27.466 | 27.482 | 27.402 | 27.447 | 27.463 | 27.479 | 27.597 | 27.589 | 27.60 |
| Qinghai | 6.594 | 6.506 | 6.528 | 6.541 | 6.588 | 6.63 | 6.661 | 6.689 | 6.755 | 6.77 | 6.789 | 6.805 | 6.804 | 6.803 | 6.846 | 6.857 | 6.93 |
| Ningxia | 8.392 | 8.383 | 8.413 | 8.41 | 8.416 | 8.429 | 8.453 | 8.536 | 8.617 | 8.644 | 8.669 | 8.661 | 8.7115 | 8.762 | 8.858 | 8.844 | 8.866 |
| Xinjiang | 28.466 | 28.558 | 28.945 | 29.062 | 29.024 | 29.067 | 29.053 | 29.123 | 29.679 | 29.675 | 29.644 | 29.654 | 29.73 | 29.806 | 29.911 | 29.962 | 30.002 |

**Table S5.** Parameter setting of PV system simulation

| Parameter Name | Description | Value in Simulation |
|---|---|---|
| Lon | Longitude of the Base station | Dependent on BSes |
| Lat | Latitude of the Base station | Dependent on BSes |
| System Capacity | Nameplate capacity (kW), converted from PV panel area | PV panel area $\times$0.16 |
| Azimuth | Azimuth angle (degrees) | 180 |
| Tile | Tile angle (degrees) | 16 |
| Losses | Total conversion loss of the system | 14.08 |

**Table S6.** Generation unit configuration in Nanchang.

| Power Plant | $N_{unit}$ | $P_i^{max}$ | $c_i^{power}$ | $c_i^{up/down}$ | $T_i^{up/down}$ |
|---|---|---|---|---|---|
| XinChang | 2 | 700 MW | 264.62 RMB/MWh | 700,000 RMB | 8 (i.e., 4 hour) |
| NanChang | 2 | 150 MW | 295.39 RMB/MWh | 150,000 RMB | 8 (i.e., 4 hour) |
| HongPing | 4 | 300 MW | 295.39 RMB/MWh | 300,000 RMB | 8 (i.e., 4 hour) |

**Table S7.** Additional carbon emissions across different provinces in China, the unit is $KtCO_2$.

| Province | Without Energy-saving | Threshold-based method | Greedy | DeepEnergy |
|---|---|---|---|---|
| Beijing | 522.607±21.703 | 305.581±11.299 | 143.671±4.287 | 4.592±0.357 |
| Tianjing | 319.228±14.464 | 185.326±7.511 | 85.617±2.208 | 2.581±0.126 |
| Hebei | 836.627±35.177 | 248.501±7.675 | 46.549±1.146 | 0.0±0.0 |
| Shanxi | 649.464±29.644 | 252.944±9.349 | 43.173±0.963 | 0.0±0.0 |
| Inner Mongolia | 434.953±17.666 | 194.915±7.172 | 37.493±0.475 | 0.0±0.0 |
| Liaoning | 368.728±14.193 | 75.564±1.668 | 16.662±2.113 | 0.0±0.0 |
| Jilin | 161.809±5.94 | 30.039±1.022 | 7.268±0.774 | 0.0±0.0 |
| Heilongjiang | 634.722±27.492 | 307.026±12.343 | 76.28±1.414 | 0.0±0.0 |
| Shanghai | 1062.309±47.839 | 710.352±29.49 | 440.367±18.228 | 56.374±0.563 |
| Jiangsu | 2536.13±116.663 | 1569.896±67.25 | 843.571±33.058 | 40.628±1.012 |
| Zhejiang | 1928.413±90.51 | 1109.701±49.74 | 502.994±22.5 | 16.555±1.273 |
| Anhui | 1004.825±47.978 | 491.846±19.35 | 128.773±3.424 | 0.781±0.413 |
| Fujian | 576.596±24.672 | 115.012±3.804 | 25.064±3.209 | 0.0±0.0 |
| Jiangxi | 1128.359±53.311 | 559.295±22.982 | 159.996±5.408 | 3.248±1.645 |
| Shandong | 1658.913±79.541 | 823.681±33.062 | 233.366±6.608 | 2.106±1.069 |
| Henan | 697.864±26.921 | 199.715±6.548 | 38.319±1.428 | 0.0±0.0 |
| Hubei | 1009.093±43.985 | 449.994±19.428 | 87.054±3.153 | 0.0±0.0 |
| Hunan | 714.896±28.868 | 236.243±7.347 | 42.25±1.844 | 0.0±0.0 |
| Guangdong | 3164.488±151.681 | 1929.178±88.293 | 1002.169±44.563 | 51.056±1.233 |
| Guangxi | 318.733±13.288 | 57.184±1.824 | 12.709±0.513 | 0.0±0.0 |
| Hainan | 188.059±7.477 | 86.129±2.185 | 17.991±0.124 | 0.0±0.0 |
| Chongqing | 563.769±23.978 | 207.374±6.858 | 35.903±1.347 | 0.0±0.0 |
| Sichuan | 386.484±14.094 | 67.572±2.084 | 11.397±5.951 | 0.0±0.0 |
| Guizhou | 848.09±39.111 | 340.227±13.72 | 60.413±1.794 | 0.0±0.0 |
| Yunnan | 1115.895±49.994 | 442.586±16.232 | 70.043±1.835 | 0.0±0.0 |
| Tibet | 18.545±0.618 | 3.877±0.512 | 0.0±0.0 | 0.0±0.0 |
| Shaanxi | 588.265±26.86 | 218.129±8.946 | 41.424±1.244 | 0.0±0.0 |
| Gansu | 76.092±2.448 | 15.973±2.469 | 1.664±0.849 | 0.0±0.0 |
| Qinghai | 44.888±1.383 | 8.16±0.169 | 1.401±0.723 | 0.0±0.0 |
| Ningxia | 157.105±6.819 | 75.137±2.41 | 18.599±0.212 | 0.0±0.0 |
| Xinjiang | 99.964±3.338 | 19.448±0.756 | 3.152±1.626 | 0.0±0.0 |
| **All over China** | **23815.926±1067.671** | **11336.618±463.515** | **4235.346±173.034** | **177.925±7.695** |

**Table S8.** Wasted energy consumption across different provinces in China, the unit is GWh.

| Province | Without Energy-saving | Threshold-based method | Greedy | DeepEnergy |
|---|---|---|---|---|
| Beijing | 768.541±9.86 | 449.383±7.888 | 211.281±5.371 | 6.754±0.826 |
| Tianjing | 469.453±4.317 | 272.539±3.869 | 125.908±3.688 | 3.796±0.394 |
| Hebei | 1230.334±14.89 | 365.443±8.676 | 68.454±2.389 | 0.0±0.0 |
| Shanxi | 955.095±8.291 | 371.977±6.621 | 63.489±2.011 | 0.0±0.0 |
| Inner Mongolia | 639.636±8.635 | 286.639±5.134 | 55.136±2.38 | 0.0±0.0 |
| Liaoning | 542.248±8.615 | 111.124±3.661 | 24.502±3.331 | 0.0±0.0 |
| Jilin | 237.954±4.282 | 44.175±0.928 | 10.688±1.298 | 0.0±0.0 |
| Heilongjiang | 933.414±10.095 | 451.508±6.473 | 112.176±4.212 | 0.0±0.0 |
| Shanghai | 1562.22±14.403 | 1044.635±13.285 | 647.599±8.571 | 82.903±5.536 |
| Jiangsu | 3729.604±30.173 | 2308.671±25.996 | 1240.545±18.747 | 59.747±2.755 |
| Zhejiang | 2835.902±20.146 | 1631.913±15.092 | 739.698±7.209 | 24.346±2.173 |
| Anhui | 1477.685±9.606 | 723.303±10.687 | 189.373±5.373 | 1.148±0.651 |
| Fujian | 847.936±9.499 | 169.135±3.574 | 36.859±4.742 | 0.0±0.0 |
| Jiangxi | 1659.351±11.434 | 822.493±10.727 | 235.288±5.016 | 4.776±2.478 |
| Shandong | 2439.578±15.449 | 1211.296±16.994 | 343.185±9.116 | 3.097±1.677 |
| Henan | 1026.27±15.899 | 293.699±6.519 | 56.352±0.96 | 0.0±0.0 |
| Hubei | 1483.96±15.383 | 661.757±7.403 | 128.02±2.37 | 0.0±0.0 |
| Hunan | 1051.317±14.455 | 347.416±8.229 | 62.132±3.356 | 0.0±0.0 |
| Guangdong | 4653.659±29.007 | 2837.027±23.849 | 1473.779±14.654 | 75.083±2.827 |
| Guangxi | 468.725±6.034 | 84.094±3.368 | 18.69±1.041 | 0.0±0.0 |
| Hainan | 276.558±4.093 | 126.661±3.758 | 26.457±1.691 | 0.0±0.0 |
| Chongqing | 829.072±9.628 | 304.962±6.567 | 52.798±0.917 | 0.0±0.0 |
| Sichuan | 568.358±10.106 | 99.371±3.609 | 16.761±8.455 | 0.0±0.0 |
| Guizhou | 1247.191±10.033 | 500.335±7.086 | 88.843±3.488 | 0.0±0.0 |
| Yunnan | 1641.022±15.189 | 650.862±11.457 | 103.005±2.847 | 0.0±0.0 |
| Tibet | 27.272±0.581 | 5.701±0.803 | 0.0±0.0 | 0.0±0.0 |
| Shaanxi | 865.096±7.42 | 320.778±4.39 | 60.918±1.449 | 0.0±0.0 |
| Gansu | 111.9±2.482 | 23.49±3.613 | 2.447±1.261 | 0.0±0.0 |
| Qinghai | 66.011±1.578 | 12.0±0.4 | 2.061±1.052 | 0.0±0.0 |
| Ningxia | 231.037±2.565 | 110.495±2.508 | 27.352±1.222 | 0.0±0.0 |
| Xinjiang | 147.006±3.19 | 28.6±0.446 | 4.635±2.365 | 0.0±0.0 |
| **All over China** | **35023.421±327.353** | **16671.497±233.626** | **6228.45±130.595** | **261.654±19.321** |

**Table S9.** Reduction in carbon emissions using different energy-saving methods across different provinces in China in 2021 compared to the case without energy-saving, the unit is $KtCO_2$.

| Province | Threshold-based method | Greedy | DeepEnergy |
|---|---|---|---|
| Beijing | 113.212±6.012 | 206.025±10.941 | 357.881±19.005 |
| Tianjing | 71.688±3.91 | 130.46±7.115 | 226.619±12.36 |
| Hebei | 381.211±20.326 | 693.736±36.989 | 1205.07±64.253 |
| Shanxi | 246.157±13.439 | 447.961±24.456 | 778.14±42.482 |
| Inner Mongolia | 143.018±7.775 | 260.267±14.15 | 452.103±24.58 |
| Liaoning | 209.421±11.318 | 381.109±20.597 | 662.014±35.779 |
| Jilin | 102.375±5.491 | 186.303±9.992 | 323.623±17.358 |
| Heilongjiang | 187.061±10.171 | 340.417±18.509 | 591.329±32.152 |
| Shanghai | 162.226±8.679 | 295.222±15.795 | 512.822±27.437 |
| Jiangsu | 500.884±26.949 | 911.519±49.042 | 1583.376±85.189 |
| Zhejiang | 446.032±23.734 | 811.698±43.192 | 1409.98±75.028 |
| Anhui | 300.536±16.031 | 546.921±29.173 | 950.043±50.675 |
| Fujian | 324.297±17.424 | 590.162±31.708 | 1025.154±55.079 |
| Jiangxi | 315.382±17.073 | 573.938±31.069 | 996.973±53.97 |
| Shandong | 491.851±26.215 | 895.08±47.706 | 1554.82±82.869 |
| Henan | 334.855±17.514 | 609.375±31.873 | 1058.529±55.365 |
| Hubei | 333.443±17.888 | 606.806±32.553 | 1054.068±56.548 |
| Hunan | 305.15±16.34 | 555.318±29.736 | 964.627±51.653 |
| Guangdong | 652.722±34.571 | 1187.837±62.913 | 2063.36±109.284 |
| Guangxi | 231.728±12.433 | 421.703±22.625 | 732.529±39.302 |
| Hainan | 59.229±3.351 | 107.787±6.098 | 187.234±10.594 |
| Chongqing | 228.378±12.447 | 415.607±22.652 | 721.94±39.348 |
| Sichuan | 441.848±23.469 | 804.083±42.709 | 1396.752±74.189 |
| Guizhou | 312.687±17.019 | 569.035±30.972 | 988.455±53.8 |
| Yunnan | 407.881±22.292 | 742.269±40.568 | 1289.377±70.47 |
| Tibet | 46.126±2.686 | 83.942±4.889 | 145.813±8.492 |
| Shaanxi | 229.54±12.256 | 417.722±22.304 | 725.613±38.744 |
| Gansu | 137.524±7.434 | 250.269±13.528 | 434.735±23.499 |
| Qinghai | 38.898±2.176 | 70.788±3.959 | 122.964±6.877 |
| Ningxia | 48.223±2.692 | 87.756±4.898 | 152.439±8.509 |
| Xinjiang | 141.318±7.684 | 257.173±13.984 | 446.729±24.29 |
| **All over China** | **7944.901±426.799** | **14458.289±776.697** | **25115.113±1349.179** |

**Table S10.** Reduction in carbon emissions using different energy-saving methods across different provinces in China in 2022 compared to the case without energy-saving, the unit is $KtCO_2$.

| **Province** | **Threshold-based method** | **Greedy** | **DeepEnergy** |
|---|---|---|---|
| Beijing | 110.464±5.769 | 201.024±10.498 | 349.193±18.236 |
| Tianjing | 70.318±3.786 | 127.967±6.89 | 222.288±11.969 |
| Hebei | 373.951±19.694 | 680.523±35.839 | 1182.118±62.255 |
| Shanxi | 242.432±13.11 | 441.182±23.859 | 766.365±41.444 |
| Inner Mongolia | 140.434±7.546 | 255.564±13.732 | 443.933±23.854 |
| Liaoning | 204.927±10.92 | 372.931±19.872 | 647.809±34.519 |
| Jilin | 99.845±5.265 | 181.7±9.581 | 315.627±16.643 |
| Heilongjiang | 184.057±9.907 | 334.95±18.03 | 581.834±31.319 |
| Shanghai | 159.727±8.459 | 290.675±15.393 | 504.924±26.739 |
| Jiangsu | 492.119±26.188 | 895.567±47.657 | 1555.666±82.784 |
| Zhejiang | 438.147±23.052 | 797.349±41.95 | 1385.054±72.87 |
| Anhui | 294.916±15.544 | 536.694±28.288 | 932.277±49.138 |
| Fujian | 319.909±17.039 | 582.176±31.009 | 1011.283±53.864 |
| Jiangxi | 311.811±16.761 | 567.44±30.503 | 985.684±52.986 |
| Shandong | 481.253±25.299 | 875.794±46.04 | 1521.32±79.975 |
| Henan | 325.137±16.669 | 591.691±30.335 | 1027.812±52.694 |
| Hubei | 328.318±17.441 | 597.479±31.74 | 1037.865±55.135 |
| Hunan | 299.22±15.816 | 544.527±28.782 | 945.883±49.997 |
| Guangdong | 638.209±33.325 | 1161.425±60.646 | 2017.482±105.346 |
| Guangxi | 225.841±11.913 | 410.991±21.68 | 713.921±37.66 |
| Hainan | 58.292±3.264 | 106.081±5.94 | 184.271±10.318 |
| Chongqing | 224.669±12.12 | 408.858±22.056 | 710.216±38.313 |
| Sichuan | 431.935±22.606 | 786.044±41.139 | 1365.416±71.461 |
| Guizhou | 308.795±16.678 | 561.952±30.352 | 976.152±52.723 |
| Yunnan | 403.642±21.921 | 734.556±39.893 | 1275.979±69.296 |
| Tibet | 45.811±2.656 | 83.368±4.834 | 144.817±8.397 |
| Shaanxi | 225.492±11.903 | 410.355±21.662 | 712.816±37.629 |
| Gansu | 134.826±7.193 | 245.359±13.089 | 426.207±22.737 |
| Qinghai | 38.235±2.113 | 69.581±3.845 | 120.867±6.679 |
| Ningxia | 47.426±2.618 | 86.307±4.765 | 149.921±8.277 |
| Xinjiang | 138.334±7.418 | 251.742±13.5 | 437.295±23.451 |
| **All over China** | **7798.493±413.996** | **14191.853±753.398** | **24652.295±1308.707** |

**Table S11.** Reduction in carbon emissions using different energy-saving methods across different provinces in China in 2023 compared to the case without energy-saving, the unit is $KtCO_2$.

| Province | Threshold-based method | Greedy | DeepEnergy |
|---|---|---|---|
| Beijing | 87.902±3.771 | 159.966±6.862 | 277.873±11.92 |
| Tianjing | 58.519±2.723 | 106.495±4.955 | 184.989±8.607 |
| Hebei | 315.702±14.624 | 574.521±26.613 | 997.986±46.228 |
| Shanxi | 211.837±10.413 | 385.505±18.95 | 669.65±32.918 |
| Inner Mongolia | 119.537±5.691 | 217.535±10.356 | 377.874±17.989 |
| Liaoning | 167.387±7.59 | 304.615±13.812 | 529.138±23.993 |
| Jilin | 79.275±3.427 | 144.267±6.237 | 250.602±10.834 |
| Heilongjiang | 158.901±7.699 | 289.17±14.011 | 502.31±24.338 |
| Shanghai | 136.175±6.378 | 247.813±11.606 | 430.47±20.16 |
| Jiangsu | 422.044±20.106 | 768.044±36.589 | 1334.149±63.558 |
| Zhejiang | 374.717±17.56 | 681.918±31.956 | 1184.542±55.51 |
| Anhui | 247.851±11.473 | 451.045±20.878 | 783.498±36.267 |
| Fujian | 282.145±13.732 | 513.453±24.99 | 891.906±43.41 |
| Jiangxi | 285.787±14.493 | 520.081±26.375 | 903.419±45.815 |
| Shandong | 398.144±18.119 | 724.551±32.974 | 1258.598±57.278 |
| Henan | 244.038±9.617 | 444.106±17.501 | 771.445±30.401 |
| Hubei | 286.491±13.795 | 521.362±25.104 | 905.645±43.608 |
| Hunan | 247.78±11.271 | 450.915±20.51 | 783.273±35.628 |
| Guangdong | 528.743±23.928 | 962.217±43.546 | 1671.442±75.642 |
| Guangxi | 178.257±7.714 | 324.397±14.039 | 563.501±24.386 |
| Hainan | 50.779±2.564 | 92.408±4.666 | 160.52±8.106 |
| Chongqing | 195.239±9.521 | 355.299±17.327 | 617.181±30.099 |
| Sichuan | 350.97±15.556 | 638.701±28.31 | 1109.471±49.176 |
| Guizhou | 279.188±14.088 | 508.071±25.638 | 882.557±44.534 |
| Yunnan | 367.085±18.719 | 668.029±34.065 | 1160.416±59.174 |
| Tibet | 43.458±2.431 | 79.086±4.425 | 137.378±7.686 |
| Shaanxi | 193.432±9.109 | 352.012±16.576 | 611.47±28.794 |
| Gansu | 111.752±5.131 | 203.369±9.337 | 353.267±16.219 |
| Qinghai | 33.082±1.626 | 60.203±2.96 | 104.578±5.142 |
| Ningxia | 41.444±2.066 | 75.42±3.76 | 131.01±6.532 |
| Xinjiang | 114.093±5.26 | 207.629±9.573 | 360.666±16.629 |
| **All over China** | **6611.755±310.196** | **12032.202±564.502** | **20900.822±980.581** |

**Table S12.** Reduction in energy consumption using different energy-saving methods across different provinces in China in 2021 compared to the case without energy-saving, the unit is GWh.

| Province | Threshold-based method | Greedy | DeepEnergy |
|---|---|---|---|
| Beijing | 166.488±0.144 | 302.978±0.262 | 526.296±0.456 |
| Tianjing | 105.424±0.06 | 191.853±0.109 | 333.263±0.19 |
| Hebei | 560.605±0.365 | 1020.2±0.664 | 1772.162±1.154 |
| Shanxi | 361.995±0.226 | 658.765±0.411 | 1144.324±0.715 |
| Inner Mongolia | 210.321±0.084 | 382.746±0.152 | 664.857±0.264 |
| Liaoning | 307.972±0.023 | 560.454±0.043 | 973.55±0.074 |
| Jilin | 150.551±0.05 | 273.976±0.092 | 475.916±0.159 |
| Heilongjiang | 275.089±0.111 | 500.613±0.202 | 869.602±0.35 |
| Shanghai | 238.568±0.112 | 434.15±0.203 | 754.151±0.353 |
| Jiangsu | 736.595±0.124 | 1340.47±0.225 | 2328.494±0.391 |
| Zhejiang | 655.93±0.498 | 1193.674±0.905 | 2073.499±1.573 |
| Anhui | 441.965±0.279 | 804.296±0.507 | 1397.121±0.881 |
| Fujian | 476.907±0.116 | 867.885±0.211 | 1507.58±0.366 |
| Jiangxi | 463.797±0.076 | 844.027±0.138 | 1466.137±0.239 |
| Shandong | 723.31±0.486 | 1316.294±0.885 | 2286.5±1.537 |
| Henan | 492.433±0.821 | 896.14±1.493 | 1556.661±2.594 |
| Hubei | 490.358±0.158 | 892.362±0.288 | 1550.099±0.501 |
| Hunan | 448.75±0.19 | 816.643±0.345 | 1418.57±0.6 |
| Guangdong | 959.886±0.966 | 1746.819±1.758 | 3034.353±3.053 |
| Guangxi | 340.776±0.108 | 620.151±0.197 | 1077.248±0.342 |
| Hainan | 87.102±0.227 | 158.51±0.414 | 275.343±0.719 |
| Chongqing | 335.85±0.179 | 611.187±0.326 | 1061.677±0.566 |
| Sichuan | 649.776±0.555 | 1182.475±1.011 | 2054.047±1.756 |
| Guizhou | 459.834±0.211 | 836.816±0.383 | 1453.611±0.666 |
| Yunnan | 599.825±0.41 | 1091.573±0.747 | 1896.142±1.297 |
| Tibet | 67.833±0.29 | 123.443±0.527 | 214.43±0.916 |
| Shaanxi | 337.559±0.194 | 614.296±0.353 | 1067.078±0.613 |
| Gansu | 202.241±0.017 | 368.042±0.031 | 639.316±0.053 |
| Qinghai | 57.204±0.112 | 104.1±0.204 | 180.83±0.354 |
| Ningxia | 70.916±0.131 | 129.053±0.239 | 224.175±0.415 |
| Xinjiang | 207.82±0.084 | 378.196±0.153 | 656.954±0.265 |
| **All over China** | **11683.678±7.406** | **21262.189±13.478** | **36933.99±23.412** |

**Table S13.** Reduction in energy consumption using different energy-saving methods across different provinces in China in 2022 compared to the case without energy-saving, the unit is MWh.

| Province | Threshold-based method | Greedy | DeepEnergy |
|---|---|---|---|
| Beijing | 162.447±0.284 | 295.624±0.517 | 513.52±0.898 |
| Tianjing | 103.41±0.013 | 188.187±0.023 | 326.894±0.041 |
| Hebei | 549.927±0.718 | 1000.769±1.307 | 1738.409±2.27 |
| Shanxi | 356.517±0.039 | 648.797±0.071 | 1127.008±0.123 |
| Inner Mongolia | 206.52±0.049 | 375.829±0.089 | 652.843±0.154 |
| Liaoning | 301.364±0.206 | 548.428±0.375 | 952.66±0.651 |
| Jilin | 146.831±0.182 | 267.206±0.331 | 464.157±0.575 |
| Heilongjiang | 270.672±0.039 | 492.574±0.07 | 855.638±0.122 |
| Shanghai | 234.893±0.238 | 427.463±0.433 | 742.535±0.752 |
| Jiangsu | 723.704±0.547 | 1317.01±0.995 | 2287.744±1.729 |
| Zhejiang | 644.334±0.876 | 1172.572±1.593 | 2036.844±2.768 |
| Anhui | 433.7±0.548 | 789.256±0.996 | 1370.995±1.731 |
| Fujian | 470.454±0.333 | 856.142±0.605 | 1487.181±1.051 |
| Jiangxi | 458.545±0.099 | 834.47±0.18 | 1449.536±0.312 |
| Shandong | 707.726±0.991 | 1287.933±1.804 | 2237.235±3.134 |
| Henan | 478.143±1.292 | 870.134±2.351 | 1511.488±4.084 |
| Hubei | 482.82±0.409 | 878.646±0.744 | 1526.273±1.292 |
| Hunan | 440.03±0.49 | 800.775±0.891 | 1391.005±1.548 |
| Guangdong | 938.543±1.646 | 1707.979±2.995 | 2966.885±5.203 |
| Guangxi | 332.12±0.405 | 604.398±0.737 | 1049.884±1.28 |
| Hainan | 85.724±0.173 | 156.002±0.315 | 270.987±0.548 |
| Chongqing | 330.396±0.008 | 601.261±0.015 | 1044.435±0.026 |
| Sichuan | 635.198±1.038 | 1155.947±1.889 | 2007.965±3.281 |
| Guizhou | 454.111±0.019 | 826.4±0.034 | 1435.517±0.059 |
| Yunnan | 593.592±0.201 | 1080.23±0.365 | 1876.439±0.635 |
| Tibet | 67.369±0.27 | 122.6±0.492 | 212.966±0.855 |
| Shaanxi | 331.606±0.392 | 603.463±0.713 | 1048.259±1.238 |
| Gansu | 198.274±0.123 | 360.823±0.225 | 626.776±0.39 |
| Qinghai | 56.228±0.073 | 102.325±0.132 | 177.746±0.23 |
| Ningxia | 69.744±0.086 | 126.922±0.157 | 220.473±0.273 |
| Xinjiang | 203.432±0.07 | 370.21±0.127 | 643.081±0.221 |
| **All over China** | **11468.373±11.854** | **20870.372±21.573** | **36253.375±37.473** |

**Table S14.** Reduction in energy consumption using different energy-saving methods across different provinces in China in 2023 compared to the case without energy-saving, the unit is GWh.

| **Province** | **Threshold-based method** | **Greedy** | **DeepEnergy** |
|---|---|---|---|
| Beijing | 129.268±1.431 | 235.244±2.604 | 408.636±4.523 |
| Tianjing | 86.058±0.64 | 156.61±1.166 | 272.043±2.025 |
| Hebei | 464.268±3.551 | 844.884±6.461 | 1467.626±11.224 |
| Shanxi | 311.525±1.499 | 566.919±2.728 | 984.78±4.738 |
| Inner Mongolia | 175.789±1.118 | 319.904±2.035 | 555.698±3.535 |
| Liaoning | 246.158±2.123 | 447.963±3.863 | 778.144±6.711 |
| Jilin | 116.581±1.252 | 212.157±2.278 | 368.532±3.957 |
| Heilongjiang | 233.677±1.289 | 425.251±2.346 | 738.692±4.076 |
| Shanghai | 200.257±1.429 | 364.431±2.6 | 633.044±4.517 |
| Jiangsu | 620.653±3.929 | 1129.476±7.149 | 1961.984±12.419 |
| Zhejiang | 551.055±3.917 | 1002.82±7.128 | 1741.973±12.381 |
| Anhui | 364.487±2.8 | 663.301±5.095 | 1152.203±8.85 |
| Fujian | 414.919±2.198 | 755.078±4.001 | 1311.626±6.95 |
| Jiangxi | 420.275±1.369 | 764.825±2.491 | 1328.557±4.326 |
| Shandong | 585.506±4.953 | 1065.516±9.014 | 1850.879±15.658 |
| Henan | 358.88±5.225 | 653.097±9.509 | 1134.477±16.519 |
| Hubei | 421.311±2.451 | 766.709±4.461 | 1331.831±7.749 |
| Hunan | 364.382±3.091 | 663.11±5.625 | 1151.872±9.77 |
| Guangdong | 777.563±6.776 | 1415.025±12.331 | 2458.003±21.419 |
| Guangxi | 262.143±2.803 | 477.054±5.1 | 828.677±8.86 |
| Hainan | 74.675±0.259 | 135.894±0.471 | 236.058±0.819 |
| Chongqing | 287.116±1.493 | 522.499±2.717 | 907.619±4.72 |
| Sichuan | 516.132±4.978 | 939.267±9.059 | 1631.576±15.736 |
| Guizhou | 410.57±1.441 | 747.164±2.622 | 1297.879±4.554 |
| Yunnan | 539.832±1.607 | 982.396±2.924 | 1706.495±5.079 |
| Tibet | 63.909±0.127 | 116.302±0.23 | 202.026±0.4 |
| Shaanxi | 284.459±1.957 | 517.664±3.561 | 899.221±6.187 |
| Gansu | 164.342±1.324 | 299.072±2.409 | 519.51±4.185 |
| Qinghai | 48.65±0.234 | 88.535±0.425 | 153.791±0.738 |
| Ningxia | 60.946±0.25 | 110.911±0.456 | 192.661±0.792 |
| Xinjiang | 167.784±1.319 | 305.336±2.401 | 530.391±4.17 |
| **All over China** | **9723.169±68.831** | **17694.415±125.26** | **30736.503±217.586** |

**Table S15.** Energy consumption of mobile networks across different province in China over years, the unit is GWh.

| Province | 2021 | 2022 | 2023 |
|---|---|---|---|
| Beijing | 1116.67±4.57 | 1130.76±5.06 | 1253.08±9.31 |
| Tianjing | 677.3±2.85 | 684.21±3.1 | 748.28±5.43 |
| Hebei | 3606.84±10.22 | 3644.1±11.45 | 3960.27±21.94 |
| Shanxi | 2263.84±7.3 | 2282.79±7.95 | 2449.12±13.66 |
| Inner Mongolia | 1339.32±4.87 | 1352.51±5.33 | 1466.14±9.3 |
| Liaoning | 1998.27±7.83 | 2021.1±8.63 | 2225.03±15.74 |
| Jilin | 1000.49±4.38 | 1013.47±4.84 | 1125.06±8.81 |
| Heilongjiang | 1746.02±6.02 | 1761.28±6.53 | 1897.93±11.17 |
| Shanghai | 1541.67±5.05 | 1554.21±5.48 | 1681.25±9.86 |
| Jiangsu | 4641.51±12.15 | 4686.25±13.62 | 5067.6±26.17 |
| Zhejiang | 4133.64±8.52 | 4173.9±9.84 | 4518.92±21.12 |
| Anhui | 2805.45±6.71 | 2833.9±7.64 | 3089.76±15.98 |
| Fujian | 2967.5±6.59 | 2989.65±7.34 | 3194.71±14.26 |
| Jiangxi | 2857.09±6.45 | 2875.7±7.07 | 3016.96±11.77 |
| Shandong | 4632.22±12.08 | 4686.5±13.85 | 5139.0±28.55 |
| Henan | 3290.93±10.12 | 3340.16±11.74 | 3781.06±26.33 |
| Hubei | 3073.59±7.21 | 3099.73±8.08 | 3327.01±15.65 |
| Hunan | 2887.99±9.2 | 2917.95±10.23 | 3197.02±19.87 |
| Guangdong | 6159.93±14.25 | 6234.9±16.64 | 6830.88±35.67 |
| Guangxi | 2214.26±7.89 | 2244.21±8.92 | 2503.33±17.83 |
| Hainan | 550.64±3.2 | 555.44±3.39 | 596.26±5.0 |
| Chongqing | 2098.21±6.55 | 2117.15±7.2 | 2277.38±12.72 |
| Sichuan | 4185.95±11.27 | 4236.27±12.94 | 4676.94±27.57 |
| Guizhou | 2831.47±7.2 | 2851.54±7.88 | 3012.65±13.29 |
| Yunnan | 3675.93±9.61 | 3697.31±10.33 | 3895.8±17.03 |
| Tibet | 407.55±2.35 | 409.2±2.42 | 421.97±2.95 |
| Shaanxi | 2149.09±5.58 | 2169.94±6.27 | 2343.94±12.07 |
| Gansu | 1298.18±4.75 | 1311.81±5.24 | 1437.1±9.69 |
| Qinghai | 360.95±1.9 | 364.38±2.04 | 392.39±3.18 |
| Ningxia | 444.71±2.12 | 448.82±2.28 | 481.4±3.54 |
| Xinjiang | 1337.87±5.36 | 1353.1±5.89 | 1484.85±10.53 |
| **All over China** | **74295.13±214.15** | **75042.23±239.24** | **81493.12±455.99** |

**Table S16.** Carbon emissions of mobile networks across different province in China over years, the unit is $KtCO_2$.

| **Province** | **2021** | **2022** | **2023** |
|---|---|---|---|
| Beijing | 759.34±44.26 | 768.92±45.13 | 852.1±52.66 |
| Tianjing | 460.57±26.9 | 465.26±27.33 | 508.83±31.35 |
| Hebei | 2452.65±139.69 | 2477.99±141.95 | 2692.99±161.07 |
| Shanxi | 1539.41±88.32 | 1552.3±89.48 | 1665.4±99.67 |
| Inner Mongolia | 910.74±52.64 | 919.71±53.46 | 996.98±60.47 |
| Liaoning | 1358.83±78.95 | 1374.35±80.36 | 1513.02±92.94 |
| Jilin | 680.33±39.86 | 689.16±40.67 | 765.04±47.6 |
| Heilongjiang | 1187.3±68.39 | 1197.67±69.32 | 1290.59±77.66 |
| Shanghai | 1048.34±60.2 | 1056.86±60.97 | 1143.25±68.77 |
| Jiangsu | 3156.23±179.05 | 3186.65±181.75 | 3445.97±204.74 |
| Zhejiang | 2810.88±157.81 | 2838.25±160.23 | 3072.87±180.98 |
| Anhui | 1907.71±107.77 | 1927.05±109.48 | 2101.04±124.85 |
| Fujian | 2017.9±113.63 | 2032.96±114.98 | 2172.41±127.46 |
| Jiangxi | 1942.82±109.48 | 1955.48±110.61 | 2051.53±119.16 |
| Shandong | 3149.91±178.66 | 3186.82±181.92 | 3494.52±209.06 |
| Henan | 2237.83±128.03 | 2271.31±131.0 | 2571.12±157.63 |
| Hubei | 2090.04±117.97 | 2107.82±119.55 | 2262.37±133.32 |
| Hunan | 1963.84±112.58 | 1984.2±114.42 | 2173.98±131.57 |
| Guangdong | 4188.75±236.28 | 4239.73±240.75 | 4645.0±276.26 |
| Guangxi | 1505.7±86.92 | 1526.06±88.76 | 1702.26±104.65 |
| Hainan | 374.44±22.5 | 377.7±22.81 | 405.46±25.47 |
| Chongqing | 1426.79±81.7 | 1439.66±82.86 | 1548.62±92.7 |
| Sichuan | 2846.44±161.7 | 2880.67±164.75 | 3180.32±191.4 |
| Guizhou | 1925.4±109.08 | 1939.05±110.3 | 2048.6±120.09 |
| Yunnan | 2499.63±141.79 | 2514.17±143.09 | 2649.15±155.18 |
| Tibet | 277.14±16.64 | 278.25±16.75 | 286.94±17.6 |
| Shaanxi | 1461.38±82.87 | 1475.56±84.13 | 1593.88±94.67 |
| Gansu | 882.76±51.05 | 892.03±51.9 | 977.23±59.69 |
| Qinghai | 245.45±14.61 | 247.78±14.83 | 266.83±16.68 |
| Ningxia | 302.4±17.84 | 305.2±18.11 | 327.35±20.2 |
| Xinjiang | 909.75±52.94 | 920.1±53.88 | 1009.69±62.04 |
| **All over China** | **50520.69±2880.11** | **51028.72±2925.51** | **55415.32±3317.61** |

**Table S17.** Data used for investment, operation and maintenance costs of photovoltaic system.

| | Component | Value | Unit |
|---|---|---|---|
| Initial investment cost | PV Modules | 3 | CNY/W |
| | Supporting structures | 0.3 | CNY/W |
| | Inverter | 0.3 | CNY/W |
| | Wirings | 0.2 | CNY/W |
| | Insurance | 0.035 | CNY/W |
| | Engineering (design, transport and assembly, installation) | 0.6 | CNY/W |
| | Junction boxes | 0.1 | CNY/W |
| Annual cost | Operation and maintenance cost | 0.03 | CNY/W |
| | Inverter replacement cost (every ten years) | 0.3 | CNY/W |
| Other details | PV panels' conversion efficiency | 16 | % |
| | Inflation rate | 3.5 | % |
| | Discount rate | 0.3 | % |
| | Lifetime of the inverter | 10 | Year |
| | Lifetime of PV System | 20 | Year |

**Table S18.** Number of base stations and $R^2$ score of estimated $M$ and ground truth in four regions.

| | **Region A** | **Region B** | **Region C** | **Region D** |
|---|---|---|---|---|
| Num of BSes | 5344 | 3439 | 2457 | 3003 |
| $R^2$ of | 0.9544 | 0.9654 | 0.9628 | 0.9537 |

**Table S19.** The $R^2$ score of estimated $M$ and ground truth of different traffic load.

| **Simulated Future Network** | $R^2$ |
|---|---|
| 40% of Capacity | 0.7800 |
| 50% of Capacity | 0.8284 |
| 60% of Capacity | 0.8701 |
| 70% of Capacity | 0.8977 |
| 80% of Capacity | 0.9211 |
| 90% of Capacity | 0.9384 |

**Table S20.** Average and standard deviation of BBU power for different types of base stations.

| Base station types | Average (W) | Standard deviation |
|---|---|---|
| 4G BS with 3 cells | 89.3771 | 5.5947 |
| 5G BS with 3 cells | 305.0409 | 26.8226 |
| 5G BS with 6 cells | 499.6484 | 44.3751 |

**Table S21.** Linear regression analysis for RRU power consumption in 5G networks.

(a) RRU power vs. transmit power in 5G networks

**Linear regression model:** $P_{RRU} = \alpha \cdot P_{trans} + \gamma$

**Dependent variable**

Transmit power ($P_{trans}$)

| **Base station types** | **Slope** ($\alpha$) | **Offset** ($\gamma$) | $R^2$ |
|---|---|---|---|
| 5G 32TR SA | 1.6928 | 389.7695 | 0.8257 |
| 5G 32TR NSA | 1.4474 | 287.3546 | 0.9595 |
| 5G 64TR SA | 1.8684 | 702.5641 | 0.7708 |
| 5G 64TR NSA | 1.6761 | 729.7315 | 0.7502 |

(b) Transmit power vs. PRB usage ratio in 5G networks

**Linear regression model:** $P_{trans} = \beta \cdot r_{PRB} + \sigma$

**Dependent variable**

PRB usage ratio ($r_{PRB}$)

| **Base station types** | **Slope** ($\beta$) | **Offset** ($\sigma$) | $R^2$ |
|---|---|---|---|
| 5G 32TR SA | 244.7592 | 0 | 0.9763 |
| 5G 32TR NSA | 259.9553 | 0 | 0.9776 |
| 5G 64TR SA | 203.0841 | 0 | 0.9599 |
| 5G 64TR NSA | 159.1848 | 0 | 0.9668 |

**Table S22.** Linear regression analysis for RRU power consumption in 4G networks.

(a) RRU power vs. transmit power in 4G networks

| **Linear regression model:** $P_{RRU} = \alpha \cdot P_{trans} + \gamma$ | | | |
|---|---|---|---|
| **Dependent variable** | | | |
| Transmit power ($P_{trans}$) | | | |
| **Base station settings** | **Slope** ($\alpha$) | **Offset** ($\gamma$) | $R^2$ |
| 4G Max transmit power: 19.87 (W) | 6.6283 | 156.6234 | 0.9471 |
| 4G Max transmit power: 39.64 (W) | 5.7572 | 138.0120 | 0.9350 |
| 4G Max transmit power: 79.09 (W) | 4.9461 | 103.0757 | 0.9690 |

(b) Transmit power vs. PRB usage ratio in 4G networks

| **Linear regression model:** $P_{trans} = \beta \cdot r_{PRB} + \sigma$ | | | |
|---|---|---|---|
| **Dependent variable** | | | |
| PRB usage ratio ($r_{PRB}$) | | | |
| **Base station settings** | **Slope** ($\alpha$) | **Offset** ($\gamma$) | $R^2$ |
| 4G Max transmit power: 19.87 (W) | 13.2436 | 6.6208 | 1.0000 |
| 4G Max transmit power: 39.64 (W) | 26.4262 | 13.2127 | 1.0000 |
| 4G Max transmit power: 79.09 (W) | 52.7272 | 26.3637 | 1.0000 |

**Table S23.** Average and standard deviation of RRU power in sleep mode for different types of base stations.

| Base station types | Average (W) | Standard deviation |
|---|---|---|
| 5G 32TR SA | 78.9992 | 8.7932 |
| 5G 32TR NSA | 69.4302 | 7.0611 |
| 5G 64TR SA | 88.4698 | 17.4029 |
| 5G 64TR NSA | 90.5637 | 11.0712 |
| 4G Max transmit power: 19.87 (W) | 119.0310 | 7.5044 |
| 4G Max transmit power: 39.64 (W) | 127.9319 | 7.6571 |
| 4G Max transmit power: 79.09 (W) | 133.9013 | 9.2278 |

**Table S24.** Parameter settings of EnergyPlus to simulation the power consumption of base stations' cooling subsystem.

| Parameters | Settings |
| --- | --- |
| Room size | 5·4·3 $m^3$ |
| Electric equipment | Communication subsystem of base stations |
| Indoor proper operating temperature | 20°C |
| Outdoor air temperature | Meteorological weather |

**Table S25.** Parameter settings of the threshold-based method used in current real-world mobile networks. (NA refers to 'not available')

| Device type | Time of a day | Metric | Sleep mode | Turn off |
|---|---|---|---|---|
| 5G cells | Nighttime (0.00am - 6.00am) | # of users | 5 | 2 |
| | | PRB usage ratio | 0.05 | 0.05 |
| | Daytime (6.00am - 11.59pm) | # of users | NA | NA |
| | | PRB usage ratio | NA | NA |
| 4G cells | Nighttime (0.00am - 6.00am) | # of users | 10 | NA |
| | | PRB usage ratio | 0.2 | NA |
| | Daytime (6.00am - 11.59pm) | # of users | 10 | NA |
| | | PRB usage ratio | 0.2 | NA |

**Table S26.** Linear regression analysis for misalignment factor.

| **Linear regression model:** $M = K_\psi(1 - \tilde{L})$ | | |
|---|---|---|
| **Dependent variable** | | |
| Normalized network traffic load $\tilde{L}$ | | |
| | | |
| **Energy-saving scenarios** | $K_\psi$ | $R^2$ |
| Without energy-saving | 0.5764 | 0.9838 |
| Threshold-based energy-saving method | 0.4765 | 0.8509 |
| Greedy energy-saving method | 0.3946 | 0.8106 |
| DeepEnergy | 0.2606 | 0.8227 |

**Table S27.** The estimated misalignment factors across provinces without energy-saving.

| Province | 2021-01 | 2021-02 | 2021-03 | 2021-04 | 2021-05 | 2021-06 | 2021-07 | 2021-08 | 2021-09 | 2021-10 | 2021-11 | 2021-12 | 2022-01 | 2022-02 | 2022-03 | 2022-04 | 2022-05 |
|---|---|---|---|---|---|---|---|---|---|---|---|---|---|---|---|---|---|
| Beijing | 0.5391±0.0031 | 0.5343±0.0031 | 0.5303±0.003 | 0.5278±0.003 | 0.526±0.003 | 0.5251±0.003 | 0.5248±0.003 | 0.5244±0.003 | 0.5237±0.003 | 0.5243±0.003 | 0.523±0.003 | 0.5216±0.003 | 0.5227±0.003 | 0.5234±0.003 | 0.5232±0.003 | 0.5221±0.003 | 0.5207±0.003 |
| Tianjing | 0.55±0.0031 | 0.5464±0.0031 | 0.5433±0.0031 | 0.5413±0.0031 | 0.5399±0.0031 | 0.5391±0.0031 | 0.5391±0.0031 | 0.5394±0.0031 | 0.539±0.0031 | 0.5391±0.0031 | 0.5382±0.0031 | 0.5374±0.0031 | 0.538±0.0031 | 0.5383±0.0031 | 0.5381±0.0031 | 0.5373±0.0031 | 0.5366±0.0031 |
| Hebei | 0.5498±0.0031 | 0.5461±0.0031 | 0.5429±0.0031 | 0.541±0.0031 | 0.5396±0.0031 | 0.5391±0.0031 | 0.5388±0.0031 | 0.5387±0.0031 | 0.5381±0.0031 | 0.5384±0.0031 | 0.5374±0.0031 | 0.5366±0.0031 | 0.5371±0.0031 | 0.5373±0.0031 | 0.5373±0.0031 | 0.5366±0.0031 | 0.5356±0.0031 |
| Shanxi | 0.5566±0.0032 | 0.5539±0.0032 | 0.5515±0.0032 | 0.5501±0.0031 | 0.5491±0.0031 | 0.5486±0.0031 | 0.5485±0.0031 | 0.5484±0.0031 | 0.548±0.0031 | 0.5483±0.0031 | 0.5477±0.0031 | 0.547±0.0031 | 0.5474±0.0031 | 0.5476±0.0031 | 0.5473±0.0031 | 0.5468±0.0031 | 0.546±0.0031 |
| Inner Mongolia | 0.5519±0.0032 | 0.5487±0.0031 | 0.5459±0.0031 | 0.5442±0.0031 | 0.5429±0.0031 | 0.5426±0.0031 | 0.5424±0.0031 | 0.5423±0.0031 | 0.542±0.0031 | 0.5422±0.0031 | 0.5413±0.0031 | 0.5404±0.0031 | 0.5409±0.0031 | 0.5412±0.0031 | 0.541±0.0031 | 0.5403±0.0031 | 0.5393±0.0031 |
| Liaoning | 0.5476±0.0031 | 0.5436±0.0031 | 0.5402±0.0031 | 0.5382±0.0031 | 0.5366±0.0031 | 0.5361±0.0031 | 0.536±0.0031 | 0.5359±0.0031 | 0.5352±0.0031 | 0.5356±0.0031 | 0.5346±0.0031 | 0.5338±0.0031 | 0.5345±0.0031 | 0.5348±0.0031 | 0.5344±0.0031 | 0.5337±0.0031 | 0.5325±0.003 |
| Jilin | 0.5419±0.0031 | 0.5373±0.0031 | 0.5332±0.0031 | 0.5307±0.003 | 0.5287±0.003 | 0.5279±0.003 | 0.5277±0.003 | 0.5277±0.003 | 0.527±0.003 | 0.5274±0.003 | 0.526±0.003 | 0.5248±0.003 | 0.5256±0.003 | 0.5259±0.003 | 0.526±0.003 | 0.5253±0.003 | 0.5236±0.003 |
| Heilongjiang | 0.5522±0.0032 | 0.5497±0.0031 | 0.5469±0.0031 | 0.5453±0.0031 | 0.544±0.0031 | 0.5436±0.0031 | 0.5436±0.0031 | 0.5436±0.0031 | 0.543±0.0031 | 0.5432±0.0031 | 0.5423±0.0031 | 0.5422±0.0031 | 0.5425±0.0031 | 0.5426±0.0031 | 0.5425±0.0031 | 0.5418±0.0031 | 0.5409±0.0031 |
| Shanghai | 0.549±0.0031 | 0.5452±0.0031 | 0.542±0.0031 | 0.5396±0.0031 | 0.5378±0.0031 | 0.5372±0.0031 | 0.537±0.0031 | 0.5369±0.0031 | 0.5365±0.0031 | 0.5367±0.0031 | 0.5357±0.0031 | 0.5356±0.0031 | 0.5362±0.0031 | 0.5364±0.0031 | 0.5364±0.0031 | 0.536±0.0031 | 0.5357±0.0031 |
| Jiangsu | 0.5548±0.0032 | 0.5518±0.0032 | 0.5492±0.0031 | 0.5477±0.0031 | 0.5465±0.0031 | 0.546±0.0031 | 0.5459±0.0031 | 0.5459±0.0031 | 0.5456±0.0031 | 0.5457±0.0031 | 0.5449±0.0031 | 0.5443±0.0031 | 0.5446±0.0031 | 0.5447±0.0031 | 0.5444±0.0031 | 0.5438±0.0031 | 0.5429±0.0031 |
| Zhejiang | 0.5548±0.0032 | 0.552±0.0032 | 0.5495±0.0031 | 0.5477±0.0031 | 0.5464±0.0031 | 0.546±0.0031 | 0.5458±0.0031 | 0.5456±0.0031 | 0.5453±0.0031 | 0.5455±0.0031 | 0.5448±0.0031 | 0.5442±0.0031 | 0.5446±0.0031 | 0.5447±0.0031 | 0.5444±0.0031 | 0.5437±0.0031 | 0.5427±0.0031 |
| Anhui | 0.5531±0.0032 | 0.5498±0.0031 | 0.5471±0.0031 | 0.5453±0.0031 | 0.5439±0.0031 | 0.5434±0.0031 | 0.5433±0.0031 | 0.5432±0.0031 | 0.5429±0.0031 | 0.5432±0.0031 | 0.5424±0.0031 | 0.5418±0.0031 | 0.5422±0.0031 | 0.5422±0.0031 | 0.542±0.0031 | 0.5414±0.0031 | 0.5404±0.0031 |
| Fujian | 0.5578±0.0032 | 0.5553±0.0032 | 0.5531±0.0032 | 0.5517±0.0032 | 0.5506±0.0032 | 0.5503±0.0032 | 0.5503±0.0032 | 0.5501±0.0031 | 0.5498±0.0031 | 0.55±0.0031 | 0.5494±0.0031 | 0.5491±0.0031 | 0.5494±0.0031 | 0.5495±0.0031 | 0.5494±0.0031 | 0.5489±0.0031 | 0.5482±0.0031 |
| Jiangxi | 0.5607±0.0032 | 0.5583±0.0032 | 0.5564±0.0032 | 0.5552±0.0032 | 0.5542±0.0032 | 0.5538±0.0032 | 0.5536±0.0032 | 0.5535±0.0032 | 0.5531±0.0032 | 0.5532±0.0032 | 0.5529±0.0032 | 0.5523±0.0032 | 0.5524±0.0032 | 0.5522±0.0032 | 0.5521±0.0032 | 0.5519±0.0032 | 0.5518±0.0032 |
| Shandong | 0.5509±0.0032 | 0.5474±0.0031 | 0.5444±0.0031 | 0.5425±0.0031 | 0.541±0.0031 | 0.5406±0.0031 | 0.5404±0.0031 | 0.5402±0.0031 | 0.5398±0.0031 | 0.5399±0.0031 | 0.5391±0.0031 | 0.5383±0.0031 | 0.5387±0.0031 | 0.5388±0.0031 | 0.5385±0.0031 | 0.5376±0.0031 | 0.5365±0.0031 |
| Henan | 0.5407±0.0031 | 0.5355±0.0031 | 0.5312±0.003 | 0.5286±0.003 | 0.5267±0.003 | 0.5259±0.003 | 0.5258±0.003 | 0.5258±0.003 | 0.5253±0.003 | 0.5255±0.003 | 0.5243±0.003 | 0.5233±0.003 | 0.5239±0.003 | 0.5241±0.003 | 0.5238±0.003 | 0.5228±0.003 | 0.5214±0.003 |
| Hubei | 0.5562±0.0032 | 0.5533±0.0032 | 0.5508±0.0032 | 0.5494±0.0031 | 0.5483±0.0031 | 0.5479±0.0031 | 0.5478±0.0031 | 0.5476±0.0031 | 0.5472±0.0031 | 0.5474±0.0031 | 0.5467±0.0031 | 0.5462±0.0031 | 0.5466±0.0031 | 0.5467±0.0031 | 0.5465±0.0031 | 0.5459±0.0031 | 0.5451±0.0031 |
| Hunan | 0.5499±0.0031 | 0.546±0.0031 | 0.5429±0.0031 | 0.5409±0.0031 | 0.5393±0.0031 | 0.5388±0.0031 | 0.5385±0.0031 | 0.5385±0.0031 | 0.538±0.0031 | 0.5383±0.0031 | 0.5375±0.0031 | 0.5368±0.0031 | 0.5374±0.0031 | 0.5377±0.0031 | 0.5376±0.0031 | 0.5368±0.0031 | 0.5357±0.0031 |
| Guangdong | 0.5506±0.0032 | 0.5472±0.0031 | 0.5442±0.0031 | 0.5419±0.0031 | 0.5405±0.0031 | 0.54±0.0031 | 0.5396±0.0031 | 0.5394±0.0031 | 0.5388±0.0031 | 0.539±0.0031 | 0.538±0.0031 | 0.5373±0.0031 | 0.5378±0.0031 | 0.538±0.0031 | 0.5374±0.0031 | 0.5364±0.0031 | 0.5353±0.0031 |
| Guangxi | 0.5475±0.0031 | 0.5432±0.0031 | 0.5398±0.0031 | 0.5377±0.0031 | 0.5362±0.0031 | 0.5358±0.0031 | 0.5355±0.0031 | 0.5352±0.0031 | 0.5347±0.0031 | 0.535±0.0031 | 0.5341±0.0031 | 0.5332±0.0031 | 0.5338±0.0031 | 0.534±0.0031 | 0.5334±0.0031 | 0.5324±0.003 | 0.531±0.003 |
| Hainan | 0.5538±0.0032 | 0.551±0.0032 | 0.5481±0.0031 | 0.5465±0.0031 | 0.5453±0.0031 | 0.545±0.0031 | 0.5451±0.0031 | 0.5451±0.0031 | 0.5443±0.0031 | 0.5444±0.0031 | 0.5437±0.0031 | 0.543±0.0031 | 0.5436±0.0031 | 0.5439±0.0031 | 0.5433±0.0031 | 0.5429±0.0031 | 0.5423±0.0031 |
| Chongqing | 0.557±0.0032 | 0.5541±0.0032 | 0.5518±0.0032 | 0.5504±0.0032 | 0.5494±0.0031 | 0.549±0.0031 | 0.5489±0.0031 | 0.5487±0.0031 | 0.5484±0.0031 | 0.5485±0.0031 | 0.5479±0.0031 | 0.5475±0.0031 | 0.5477±0.0031 | 0.5476±0.0031 | 0.5474±0.0031 | 0.5468±0.0031 | 0.546±0.0031 |
| Sichuan | 0.5494±0.0031 | 0.5455±0.0031 | 0.5423±0.0031 | 0.5406±0.0031 | 0.5391±0.0031 | 0.5383±0.0031 | 0.5382±0.0031 | 0.5382±0.0031 | 0.5379±0.0031 | 0.5382±0.0031 | 0.5373±0.0031 | 0.5364±0.0031 | 0.5369±0.0031 | 0.537±0.0031 | 0.5366±0.0031 | 0.5357±0.0031 | 0.5347±0.0031 |
| Guizhou | 0.5605±0.0032 | 0.5582±0.0032 | 0.5563±0.0032 | 0.5552±0.0032 | 0.5543±0.0032 | 0.5541±0.0032 | 0.554±0.0032 | 0.5537±0.0032 | 0.5535±0.0032 | 0.5536±0.0032 | 0.553±0.0032 | 0.5524±0.0032 | 0.5527±0.0032 | 0.5528±0.0032 | 0.5526±0.0032 | 0.5522±0.0032 | 0.5515±0.0032 |
| Yunnan | 0.5615±0.0032 | 0.5594±0.0032 | 0.5576±0.0032 | 0.5566±0.0032 | 0.5559±0.0032 | 0.5557±0.0032 | 0.5555±0.0032 | 0.5554±0.0032 | 0.5552±0.0032 | 0.5554±0.0032 | 0.5549±0.0032 | 0.5545±0.0032 | 0.5548±0.0032 | 0.555±0.0032 | 0.5549±0.0032 | 0.5545±0.0032 | 0.554±0.0032 |
| Tibet | 0.5664±0.0032 | 0.5652±0.0032 | 0.5642±0.0032 | 0.5632±0.0032 | 0.5627±0.0032 | 0.5625±0.0032 | 0.5623±0.0032 | 0.5623±0.0032 | 0.562±0.0032 | 0.562±0.0032 | 0.5617±0.0032 | 0.5614±0.0032 | 0.5616±0.0032 | 0.5618±0.0032 | 0.5616±0.0032 | 0.5613±0.0032 | 0.5609±0.0032 |
| Shaanxi | 0.5524±0.0032 | 0.5493±0.0031 | 0.5467±0.0031 | 0.5446±0.0031 | 0.5432±0.0031 | 0.5425±0.0031 | 0.5422±0.0031 | 0.542±0.0031 | 0.5416±0.0031 | 0.5418±0.0031 | 0.541±0.0031 | 0.5403±0.0031 | 0.5409±0.0031 | 0.5411±0.0031 | 0.5406±0.0031 | 0.5402±0.0031 | 0.5392±0.0031 |
| Gansu | 0.5504±0.0032 | 0.5468±0.0031 | 0.5436±0.0031 | 0.5417±0.0031 | 0.5401±0.0031 | 0.5396±0.0031 | 0.5395±0.0031 | 0.5394±0.0031 | 0.5389±0.0031 | 0.5393±0.0031 | 0.5385±0.0031 | 0.5377±0.0031 | 0.5383±0.0031 | 0.5385±0.0031 | 0.5383±0.0031 | 0.5376±0.0031 | 0.5366±0.0031 |
| Qinghai | 0.5544±0.0032 | 0.5516±0.0032 | 0.5491±0.0031 | 0.5475±0.0031 | 0.5461±0.0031 | 0.5456±0.0031 | 0.5454±0.0031 | 0.5453±0.0031 | 0.5448±0.0031 | 0.545±0.0031 | 0.5442±0.0031 | 0.5435±0.0031 | 0.544±0.0031 | 0.5442±0.0031 | 0.544±0.0031 | 0.5433±0.0031 | 0.5421±0.0031 |
| Ningxia | 0.556±0.0032 | 0.5531±0.0032 | 0.5508±0.0032 | 0.5493±0.0031 | 0.5482±0.0031 | 0.5479±0.0031 | 0.5477±0.0031 | 0.5475±0.0031 | 0.547±0.0031 | 0.5472±0.0031 | 0.5464±0.0031 | 0.5459±0.0031 | 0.5462±0.0031 | 0.5462±0.0031 | 0.5458±0.0031 | 0.5453±0.0031 | 0.5444±0.0031 |
| Xinjiang | 0.5499±0.0031 | 0.5461±0.0031 | 0.5427±0.0031 | 0.5406±0.0031 | 0.5392±0.0031 | 0.5388±0.0031 | 0.5387±0.0031 | 0.5387±0.0031 | 0.5377±0.0031 | 0.5381±0.0031 | 0.5372±0.0031 | 0.5365±0.0031 | 0.537±0.0031 | 0.5371±0.0031 | 0.5369±0.0031 | 0.5361±0.0031 | 0.535±0.0031 |

**Table S28.** The estimated misalignment factors across provinces with threshold-based energy-saving method.

| Province | 2021-01 | 2021-02 | 2021-03 | 2021-04 | 2021-05 | 2021-06 | 2021-07 | 2021-08 | 2021-09 | 2021-10 | 2021-11 | 2021-12 | 2022-01 | 2022-02 | 2022-03 | 2022-04 | 2022-05 |
|---|---|---|---|---|---|---|---|---|---|---|---|---|---|---|---|---|---|
| Beijing | 0.4457±0.0064 | 0.4417±0.0063 | 0.4384±0.0063 | 0.4364±0.0062 | 0.4348±0.0062 | 0.4341±0.0062 | 0.4339±0.0062 | 0.4335±0.0062 | 0.4329±0.0062 | 0.4335±0.0062 | 0.4323±0.0062 | 0.4312±0.0062 | 0.4321±0.0062 | 0.4326±0.0062 | 0.4325±0.0062 | 0.4316±0.0062 | 0.4305±0.0061 |
| Tianjing | 0.4547±0.0065 | 0.4517±0.0064 | 0.4491±0.0064 | 0.4475±0.0064 | 0.4463±0.0064 | 0.4457±0.0064 | 0.4457±0.0064 | 0.4459±0.0064 | 0.4456±0.0064 | 0.4456±0.0064 | 0.4449±0.0063 | 0.4443±0.0063 | 0.4448±0.0063 | 0.445±0.0064 | 0.4449±0.0063 | 0.4442±0.0063 | 0.4436±0.0063 |
| Hebei | 0.4545±0.0065 | 0.4514±0.0064 | 0.4488±0.0064 | 0.4472±0.0064 | 0.446±0.0064 | 0.4456±0.0064 | 0.4454±0.0064 | 0.4453±0.0064 | 0.4449±0.0063 | 0.4451±0.0064 | 0.4443±0.0063 | 0.4436±0.0063 | 0.444±0.0063 | 0.4442±0.0063 | 0.4442±0.0063 | 0.4436±0.0063 | 0.4428±0.0063 |
| Shanxi | 0.4601±0.0066 | 0.4579±0.0065 | 0.4559±0.0065 | 0.4548±0.0065 | 0.4539±0.0065 | 0.4535±0.0065 | 0.4535±0.0065 | 0.4534±0.0065 | 0.4531±0.0065 | 0.4533±0.0065 | 0.4527±0.0065 | 0.4522±0.0065 | 0.4526±0.0065 | 0.4527±0.0065 | 0.4525±0.0065 | 0.452±0.0065 | 0.4514±0.0064 |
| Inner Mongolia | 0.4563±0.0065 | 0.4536±0.0065 | 0.4513±0.0064 | 0.4499±0.0064 | 0.4488±0.0064 | 0.4485±0.0064 | 0.4484±0.0064 | 0.4483±0.0064 | 0.448±0.0064 | 0.4483±0.0064 | 0.4475±0.0064 | 0.4467±0.0064 | 0.4472±0.0064 | 0.4474±0.0064 | 0.4472±0.0064 | 0.4466±0.0064 | 0.4458±0.0064 |
| Liaoning | 0.4527±0.0065 | 0.4494±0.0064 | 0.4466±0.0064 | 0.4449±0.0063 | 0.4436±0.0063 | 0.4432±0.0063 | 0.4431±0.0063 | 0.443±0.0063 | 0.4425±0.0063 | 0.4427±0.0063 | 0.442±0.0063 | 0.4413±0.0063 | 0.4418±0.0063 | 0.4421±0.0063 | 0.4418±0.0063 | 0.4412±0.0063 | 0.4402±0.0063 |
| Jilin | 0.448±0.0064 | 0.4442±0.0063 | 0.4408±0.0063 | 0.4387±0.0063 | 0.437±0.0062 | 0.4364±0.0062 | 0.4363±0.0062 | 0.4362±0.0062 | 0.4357±0.0062 | 0.436±0.0062 | 0.4348±0.0062 | 0.4339±0.0062 | 0.4345±0.0062 | 0.4348±0.0062 | 0.4348±0.0062 | 0.4343±0.0062 | 0.4328±0.0062 |
| Heilongjiang | 0.4565±0.0065 | 0.4544±0.0065 | 0.4521±0.0065 | 0.4508±0.0064 | 0.4497±0.0064 | 0.4494±0.0064 | 0.4494±0.0064 | 0.4494±0.0064 | 0.4489±0.0064 | 0.449±0.0064 | 0.4483±0.0064 | 0.4482±0.0064 | 0.4485±0.0064 | 0.4486±0.0064 | 0.4485±0.0064 | 0.4479±0.0064 | 0.4471±0.0064 |
| Shanghai | 0.4538±0.0065 | 0.4507±0.0064 | 0.448±0.0064 | 0.4461±0.0064 | 0.4446±0.0063 | 0.4441±0.0063 | 0.4439±0.0063 | 0.4438±0.0063 | 0.4435±0.0063 | 0.4437±0.0063 | 0.4429±0.0063 | 0.4428±0.0063 | 0.4433±0.0063 | 0.4435±0.0063 | 0.4434±0.0063 | 0.4431±0.0063 | 0.4429±0.0063 |
| Jiangsu | 0.4586±0.0065 | 0.4561±0.0065 | 0.454±0.0065 | 0.4527±0.0065 | 0.4517±0.0064 | 0.4514±0.0064 | 0.4513±0.0064 | 0.4513±0.0064 | 0.451±0.0064 | 0.4511±0.0064 | 0.4505±0.0064 | 0.4499±0.0064 | 0.4502±0.0064 | 0.4503±0.0064 | 0.4501±0.0064 | 0.4496±0.0064 | 0.4488±0.0064 |
| Zhejiang | 0.4587±0.0065 | 0.4564±0.0065 | 0.4542±0.0065 | 0.4527±0.0065 | 0.4517±0.0064 | 0.4514±0.0064 | 0.4512±0.0064 | 0.4511±0.0064 | 0.4508±0.0064 | 0.4509±0.0064 | 0.4504±0.0064 | 0.4499±0.0064 | 0.4502±0.0064 | 0.4503±0.0064 | 0.45±0.0064 | 0.4495±0.0064 | 0.4487±0.0064 |
| Anhui | 0.4573±0.0065 | 0.4545±0.0065 | 0.4522±0.0065 | 0.4508±0.0064 | 0.4496±0.0064 | 0.4492±0.0064 | 0.4491±0.0064 | 0.449±0.0064 | 0.4488±0.0064 | 0.449±0.0064 | 0.4484±0.0064 | 0.4479±0.0064 | 0.4482±0.0064 | 0.4482±0.0064 | 0.4481±0.0064 | 0.4475±0.0064 | 0.4468±0.0064 |
| Fujian | 0.4611±0.0066 | 0.459±0.0066 | 0.4572±0.0065 | 0.4561±0.0065 | 0.4552±0.0065 | 0.4549±0.0065 | 0.4549±0.0065 | 0.4548±0.0065 | 0.4545±0.0065 | 0.4547±0.0065 | 0.4542±0.0065 | 0.4539±0.0065 | 0.4542±0.0065 | 0.4543±0.0065 | 0.4542±0.0065 | 0.4537±0.0065 | 0.4532±0.0065 |
| Jiangxi | 0.4635±0.0066 | 0.4615±0.0066 | 0.4599±0.0066 | 0.459±0.0065 | 0.4582±0.0065 | 0.4578±0.0065 | 0.4577±0.0065 | 0.4575±0.0065 | 0.4572±0.0065 | 0.4573±0.0065 | 0.4571±0.0065 | 0.4566±0.0065 | 0.4566±0.0065 | 0.4565±0.0065 | 0.4564±0.0065 | 0.4562±0.0065 | 0.4561±0.0065 |
| Shandong | 0.4554±0.0065 | 0.4525±0.0065 | 0.4501±0.0064 | 0.4485±0.0064 | 0.4472±0.0064 | 0.4469±0.0064 | 0.4467±0.0064 | 0.4466±0.0064 | 0.4463±0.0064 | 0.4464±0.0064 | 0.4457±0.0064 | 0.445±0.0064 | 0.4454±0.0064 | 0.4454±0.0064 | 0.4452±0.0064 | 0.4445±0.0063 | 0.4435±0.0063 |
| Henan | 0.447±0.0064 | 0.4427±0.0063 | 0.4391±0.0063 | 0.437±0.0062 | 0.4354±0.0062 | 0.4348±0.0062 | 0.4346±0.0062 | 0.4347±0.0062 | 0.4343±0.0062 | 0.4344±0.0062 | 0.4334±0.0062 | 0.4326±0.0062 | 0.4331±0.0062 | 0.4333±0.0062 | 0.4331±0.0062 | 0.4322±0.0062 | 0.431±0.0062 |
| Hubei | 0.4598±0.0066 | 0.4574±0.0065 | 0.4554±0.0065 | 0.4542±0.0065 | 0.4533±0.0065 | 0.4529±0.0065 | 0.4529±0.0065 | 0.4527±0.0065 | 0.4524±0.0065 | 0.4525±0.0065 | 0.4519±0.0064 | 0.4516±0.0064 | 0.4519±0.0064 | 0.452±0.0064 | 0.4518±0.0064 | 0.4513±0.0064 | 0.4506±0.0064 |
| Hunan | 0.4546±0.0065 | 0.4514±0.0064 | 0.4488±0.0064 | 0.4472±0.0064 | 0.4458±0.0064 | 0.4454±0.0064 | 0.4452±0.0064 | 0.4452±0.0064 | 0.4447±0.0063 | 0.445±0.0064 | 0.4444±0.0063 | 0.4437±0.0063 | 0.4443±0.0063 | 0.4445±0.0063 | 0.4444±0.0063 | 0.4438±0.0063 | 0.4429±0.0063 |
| Guangdong | 0.4551±0.0065 | 0.4524±0.0065 | 0.4499±0.0064 | 0.448±0.0064 | 0.4468±0.0064 | 0.4464±0.0064 | 0.4461±0.0064 | 0.4459±0.0064 | 0.4455±0.0064 | 0.4456±0.0064 | 0.4448±0.0063 | 0.4441±0.0063 | 0.4446±0.0063 | 0.4448±0.0063 | 0.4442±0.0063 | 0.4435±0.0063 | 0.4425±0.0063 |
| Guangxi | 0.4526±0.0065 | 0.4491±0.0064 | 0.4462±0.0064 | 0.4445±0.0063 | 0.4433±0.0063 | 0.4429±0.0063 | 0.4427±0.0063 | 0.4424±0.0063 | 0.442±0.0063 | 0.4423±0.0063 | 0.4415±0.0063 | 0.4408±0.0063 | 0.4413±0.0063 | 0.4414±0.0063 | 0.4409±0.0063 | 0.4401±0.0063 | 0.439±0.0063 |
| Hainan | 0.4578±0.0065 | 0.4555±0.0065 | 0.4531±0.0065 | 0.4518±0.0064 | 0.4508±0.0064 | 0.4506±0.0064 | 0.4506±0.0064 | 0.4506±0.0064 | 0.45±0.0064 | 0.4501±0.0064 | 0.4495±0.0064 | 0.4489±0.0064 | 0.4494±0.0064 | 0.4496±0.0064 | 0.4491±0.0064 | 0.4488±0.0064 | 0.4483±0.0064 |
| Chongqing | 0.4605±0.0066 | 0.4581±0.0065 | 0.4562±0.0065 | 0.455±0.0065 | 0.4541±0.0065 | 0.4539±0.0065 | 0.4538±0.0065 | 0.4536±0.0065 | 0.4533±0.0065 | 0.4535±0.0065 | 0.453±0.0065 | 0.4526±0.0065 | 0.4527±0.0065 | 0.4527±0.0065 | 0.4525±0.0065 | 0.4521±0.0065 | 0.4514±0.0064 |
| Sichuan | 0.4542±0.0065 | 0.451±0.0064 | 0.4483±0.0064 | 0.4469±0.0064 | 0.4457±0.0064 | 0.445±0.0064 | 0.4449±0.0063 | 0.4449±0.0063 | 0.4447±0.0063 | 0.4449±0.0063 | 0.4441±0.0063 | 0.4435±0.0063 | 0.4438±0.0063 | 0.4439±0.0063 | 0.4436±0.0063 | 0.4429±0.0063 | 0.442±0.0063 |
| Guizhou | 0.4634±0.0066 | 0.4615±0.0066 | 0.4599±0.0066 | 0.459±0.0065 | 0.4583±0.0065 | 0.458±0.0065 | 0.458±0.0065 | 0.4577±0.0065 | 0.4575±0.0065 | 0.4576±0.0065 | 0.4572±0.0065 | 0.4567±0.0065 | 0.4569±0.0065 | 0.457±0.0065 | 0.4568±0.0065 | 0.4565±0.0065 | 0.4559±0.0065 |
| Yunnan | 0.4642±0.0066 | 0.4624±0.0066 | 0.4609±0.0066 | 0.4601±0.0066 | 0.4596±0.0066 | 0.4593±0.0066 | 0.4592±0.0066 | 0.4591±0.0066 | 0.459±0.0065 | 0.4592±0.0066 | 0.4588±0.0065 | 0.4584±0.0065 | 0.4587±0.0065 | 0.4588±0.0065 | 0.4587±0.0065 | 0.4584±0.0065 | 0.4579±0.0065 |
| Tibet | 0.4682±0.0067 | 0.4672±0.0067 | 0.4664±0.0067 | 0.4656±0.0066 | 0.4652±0.0066 | 0.465±0.0066 | 0.4649±0.0066 | 0.4648±0.0066 | 0.4646±0.0066 | 0.4646±0.0066 | 0.4644±0.0066 | 0.4641±0.0066 | 0.4643±0.0066 | 0.4644±0.0066 | 0.4643±0.0066 | 0.464±0.0066 | 0.4637±0.0066 |
| Shaanxi | 0.4567±0.0065 | 0.4541±0.0065 | 0.452±0.0064 | 0.4502±0.0064 | 0.449±0.0064 | 0.4484±0.0064 | 0.4482±0.0064 | 0.4481±0.0064 | 0.4478±0.0064 | 0.4479±0.0064 | 0.4472±0.0064 | 0.4467±0.0064 | 0.4471±0.0064 | 0.4474±0.0064 | 0.4469±0.0064 | 0.4466±0.0064 | 0.4458±0.0064 |
| Gansu | 0.455±0.0065 | 0.452±0.0065 | 0.4494±0.0064 | 0.4478±0.0064 | 0.4465±0.0064 | 0.4461±0.0064 | 0.446±0.0064 | 0.4459±0.0064 | 0.4455±0.0064 | 0.4458±0.0064 | 0.4452±0.0064 | 0.4445±0.0063 | 0.445±0.0064 | 0.4452±0.0064 | 0.445±0.0064 | 0.4444±0.0063 | 0.4436±0.0063 |
| Qinghai | 0.4583±0.0065 | 0.456±0.0065 | 0.4539±0.0065 | 0.4526±0.0065 | 0.4515±0.0064 | 0.451±0.0064 | 0.4509±0.0064 | 0.4508±0.0064 | 0.4504±0.0064 | 0.4506±0.0064 | 0.4499±0.0064 | 0.4493±0.0064 | 0.4497±0.0064 | 0.4499±0.0064 | 0.4497±0.0064 | 0.4491±0.0064 | 0.4481±0.0064 |
| Ningxia | 0.4596±0.0066 | 0.4573±0.0065 | 0.4553±0.0065 | 0.4541±0.0065 | 0.4532±0.0065 | 0.4529±0.0065 | 0.4528±0.0065 | 0.4526±0.0065 | 0.4522±0.0065 | 0.4523±0.0065 | 0.4517±0.0064 | 0.4513±0.0064 | 0.4515±0.0064 | 0.4515±0.0064 | 0.4512±0.0064 | 0.4508±0.0064 | 0.4501±0.0064 |
| Xinjiang | 0.4546±0.0065 | 0.4514±0.0064 | 0.4486±0.0064 | 0.4469±0.0064 | 0.4458±0.0064 | 0.4454±0.0064 | 0.4454±0.0064 | 0.4453±0.0064 | 0.4445±0.0063 | 0.4448±0.0063 | 0.4441±0.0063 | 0.4435±0.0063 | 0.4439±0.0063 | 0.444±0.0063 | 0.4439±0.0063 | 0.4432±0.0063 | 0.4423±0.0063 |

**Table S29.** The estimated misalignment factors across provinces with greedy energy-saving method.

| Province | 2021-01 | 2021-02 | 2021-03 | 2021-04 | 2021-05 | 2021-06 | 2021-07 | 2021-08 | 2021-09 | 2021-10 | 2021-11 | 2021-12 | 2022-01 | 2022-02 | 2022-03 | 2022-04 | 2022-05 |
|---|---|---|---|---|---|---|---|---|---|---|---|---|---|---|---|---|---|
| Beijing | 0.3691±0.0048 | 0.3658±0.0047 | 0.363±0.0047 | 0.3614±0.0047 | 0.3601±0.0047 | 0.3595±0.0046 | 0.3593±0.0046 | 0.359±0.0046 | 0.3585±0.0046 | 0.359±0.0046 | 0.358±0.0046 | 0.3571±0.0046 | 0.3578±0.0046 | 0.3583±0.0046 | 0.3582±0.0046 | 0.3574±0.0046 | 0.3565±0.0046 |
| Tianjing | 0.3765±0.0049 | 0.374±0.0048 | 0.3719±0.0048 | 0.3706±0.0048 | 0.3696±0.0048 | 0.3691±0.0048 | 0.3691±0.0048 | 0.3692±0.0048 | 0.369±0.0048 | 0.369±0.0048 | 0.3684±0.0048 | 0.3679±0.0048 | 0.3683±0.0048 | 0.3685±0.0048 | 0.3684±0.0048 | 0.3678±0.0048 | 0.3673±0.0047 |
| Hebei | 0.3764±0.0049 | 0.3738±0.0048 | 0.3717±0.0048 | 0.3704±0.0048 | 0.3694±0.0048 | 0.369±0.0048 | 0.3689±0.0048 | 0.3688±0.0048 | 0.3684±0.0048 | 0.3686±0.0048 | 0.3679±0.0048 | 0.3673±0.0047 | 0.3677±0.0048 | 0.3678±0.0048 | 0.3678±0.0048 | 0.3673±0.0047 | 0.3667±0.0047 |
| Shanxi | 0.381±0.0049 | 0.3792±0.0049 | 0.3776±0.0049 | 0.3766±0.0049 | 0.3759±0.0049 | 0.3756±0.0049 | 0.3755±0.0049 | 0.3755±0.0049 | 0.3752±0.0048 | 0.3754±0.0049 | 0.3749±0.0048 | 0.3745±0.0048 | 0.3748±0.0048 | 0.3749±0.0048 | 0.3747±0.0048 | 0.3743±0.0048 | 0.3738±0.0048 |
| Inner Mongolia | 0.3779±0.0049 | 0.3756±0.0049 | 0.3737±0.0048 | 0.3725±0.0048 | 0.3717±0.0048 | 0.3714±0.0048 | 0.3714±0.0048 | 0.3713±0.0048 | 0.371±0.0048 | 0.3712±0.0048 | 0.3705±0.0048 | 0.3699±0.0048 | 0.3703±0.0048 | 0.3705±0.0048 | 0.3704±0.0048 | 0.3699±0.0048 | 0.3692±0.0048 |
| Liaoning | 0.3749±0.0048 | 0.3722±0.0048 | 0.3698±0.0048 | 0.3684±0.0048 | 0.3674±0.0047 | 0.367±0.0047 | 0.3669±0.0047 | 0.3669±0.0047 | 0.3664±0.0047 | 0.3666±0.0047 | 0.366±0.0047 | 0.3654±0.0047 | 0.3659±0.0047 | 0.3661±0.0047 | 0.3658±0.0047 | 0.3654±0.0047 | 0.3645±0.0047 |
| Jilin | 0.371±0.0048 | 0.3678±0.0048 | 0.365±0.0047 | 0.3633±0.0047 | 0.3619±0.0047 | 0.3614±0.0047 | 0.3613±0.0047 | 0.3612±0.0047 | 0.3608±0.0047 | 0.3611±0.0047 | 0.3601±0.0047 | 0.3593±0.0046 | 0.3598±0.0047 | 0.36±0.0047 | 0.3601±0.0047 | 0.3596±0.0046 | 0.3584±0.0046 |
| Heilongjiang | 0.378±0.0049 | 0.3763±0.0049 | 0.3744±0.0048 | 0.3733±0.0048 | 0.3724±0.0048 | 0.3722±0.0048 | 0.3722±0.0048 | 0.3721±0.0048 | 0.3718±0.0048 | 0.3719±0.0048 | 0.3713±0.0048 | 0.3712±0.0048 | 0.3714±0.0048 | 0.3715±0.0048 | 0.3714±0.0048 | 0.3709±0.0048 | 0.3703±0.0048 |
| Shanghai | 0.3758±0.0049 | 0.3732±0.0048 | 0.371±0.0048 | 0.3694±0.0048 | 0.3682±0.0048 | 0.3678±0.0048 | 0.3676±0.0048 | 0.3675±0.0048 | 0.3673±0.0047 | 0.3674±0.0047 | 0.3668±0.0047 | 0.3667±0.0047 | 0.3671±0.0047 | 0.3672±0.0047 | 0.3672±0.0047 | 0.367±0.0047 | 0.3667±0.0047 |
| Jiangsu | 0.3798±0.0049 | 0.3777±0.0049 | 0.376±0.0049 | 0.3749±0.0048 | 0.3741±0.0048 | 0.3738±0.0048 | 0.3737±0.0048 | 0.3737±0.0048 | 0.3735±0.0048 | 0.3736±0.0048 | 0.3731±0.0048 | 0.3726±0.0048 | 0.3728±0.0048 | 0.3729±0.0048 | 0.3727±0.0048 | 0.3723±0.0048 | 0.3717±0.0048 |
| Zhejiang | 0.3798±0.0049 | 0.3779±0.0049 | 0.3762±0.0049 | 0.3749±0.0048 | 0.3741±0.0048 | 0.3738±0.0048 | 0.3737±0.0048 | 0.3735±0.0048 | 0.3733±0.0048 | 0.3734±0.0048 | 0.373±0.0048 | 0.3726±0.0048 | 0.3728±0.0048 | 0.3729±0.0048 | 0.3727±0.0048 | 0.3722±0.0048 | 0.3716±0.0048 |
| Anhui | 0.3787±0.0049 | 0.3764±0.0049 | 0.3745±0.0048 | 0.3733±0.0048 | 0.3723±0.0048 | 0.372±0.0048 | 0.3719±0.0048 | 0.3719±0.0048 | 0.3716±0.0048 | 0.3718±0.0048 | 0.3713±0.0048 | 0.3709±0.0048 | 0.3712±0.0048 | 0.3712±0.0048 | 0.3711±0.0048 | 0.3706±0.0048 | 0.37±0.0048 |
| Fujian | 0.3819±0.0049 | 0.3801±0.0049 | 0.3786±0.0049 | 0.3777±0.0049 | 0.377±0.0049 | 0.3767±0.0049 | 0.3767±0.0049 | 0.3766±0.0049 | 0.3764±0.0049 | 0.3766±0.0049 | 0.3761±0.0049 | 0.3759±0.0049 | 0.3761±0.0049 | 0.3762±0.0049 | 0.3761±0.0049 | 0.3758±0.0049 | 0.3753±0.0049 |
| Jiangxi | 0.3838±0.005 | 0.3822±0.0049 | 0.3809±0.0049 | 0.3801±0.0049 | 0.3794±0.0049 | 0.3791±0.0049 | 0.379±0.0049 | 0.3789±0.0049 | 0.3786±0.0049 | 0.3787±0.0049 | 0.3785±0.0049 | 0.3781±0.0049 | 0.3781±0.0049 | 0.378±0.0049 | 0.3779±0.0049 | 0.3778±0.0049 | 0.3777±0.0049 |
| Shandong | 0.3771±0.0049 | 0.3748±0.0048 | 0.3727±0.0048 | 0.3714±0.0048 | 0.3704±0.0048 | 0.3701±0.0048 | 0.3699±0.0048 | 0.3698±0.0048 | 0.3696±0.0048 | 0.3696±0.0048 | 0.3691±0.0048 | 0.3685±0.0048 | 0.3688±0.0048 | 0.3689±0.0048 | 0.3686±0.0048 | 0.3681±0.0048 | 0.3673±0.0047 |
| Henan | 0.3702±0.0048 | 0.3666±0.0047 | 0.3637±0.0047 | 0.3619±0.0047 | 0.3605±0.0047 | 0.36±0.0047 | 0.3599±0.0047 | 0.36±0.0047 | 0.3596±0.0046 | 0.3597±0.0046 | 0.3589±0.0046 | 0.3582±0.0046 | 0.3587±0.0046 | 0.3588±0.0046 | 0.3586±0.0046 | 0.3579±0.0046 | 0.3569±0.0046 |
| Hubei | 0.3808±0.0049 | 0.3788±0.0049 | 0.3771±0.0049 | 0.3761±0.0049 | 0.3754±0.0049 | 0.3751±0.0048 | 0.375±0.0048 | 0.3749±0.0048 | 0.3746±0.0048 | 0.3747±0.0048 | 0.3742±0.0048 | 0.3739±0.0048 | 0.3742±0.0048 | 0.3743±0.0048 | 0.3742±0.0048 | 0.3737±0.0048 | 0.3732±0.0048 |
| Hunan | 0.3764±0.0049 | 0.3738±0.0048 | 0.3717±0.0048 | 0.3703±0.0048 | 0.3692±0.0048 | 0.3689±0.0048 | 0.3687±0.0048 | 0.3687±0.0048 | 0.3683±0.0048 | 0.3685±0.0048 | 0.368±0.0048 | 0.3675±0.0047 | 0.3679±0.0048 | 0.3681±0.0048 | 0.368±0.0048 | 0.3675±0.0047 | 0.3668±0.0047 |
| Guangdong | 0.3769±0.0049 | 0.3746±0.0048 | 0.3726±0.0048 | 0.371±0.0048 | 0.37±0.0048 | 0.3697±0.0048 | 0.3694±0.0048 | 0.3693±0.0048 | 0.3689±0.0048 | 0.369±0.0048 | 0.3683±0.0048 | 0.3678±0.0048 | 0.3682±0.0048 | 0.3683±0.0048 | 0.3679±0.0048 | 0.3672±0.0047 | 0.3665±0.0047 |
| Guangxi | 0.3748±0.0048 | 0.3719±0.0048 | 0.3695±0.0048 | 0.3681±0.0048 | 0.3671±0.0047 | 0.3668±0.0047 | 0.3666±0.0047 | 0.3664±0.0047 | 0.3661±0.0047 | 0.3662±0.0047 | 0.3656±0.0047 | 0.3651±0.0047 | 0.3654±0.0047 | 0.3656±0.0047 | 0.3651±0.0047 | 0.3645±0.0047 | 0.3635±0.0047 |
| Hainan | 0.3791±0.0049 | 0.3772±0.0049 | 0.3752±0.0048 | 0.3741±0.0048 | 0.3733±0.0048 | 0.3731±0.0048 | 0.3732±0.0048 | 0.3732±0.0048 | 0.3726±0.0048 | 0.3727±0.0048 | 0.3722±0.0048 | 0.3717±0.0048 | 0.3721±0.0048 | 0.3723±0.0048 | 0.3719±0.0048 | 0.3717±0.0048 | 0.3712±0.0048 |
| Chongqing | 0.3813±0.0049 | 0.3793±0.0049 | 0.3778±0.0049 | 0.3768±0.0049 | 0.3761±0.0049 | 0.3759±0.0049 | 0.3758±0.0049 | 0.3757±0.0049 | 0.3754±0.0049 | 0.3755±0.0049 | 0.3751±0.0048 | 0.3748±0.0048 | 0.3749±0.0048 | 0.3749±0.0048 | 0.3748±0.0048 | 0.3744±0.0048 | 0.3738±0.0048 |
| Sichuan | 0.3761±0.0049 | 0.3735±0.0048 | 0.3713±0.0048 | 0.3701±0.0048 | 0.3691±0.0048 | 0.3685±0.0048 | 0.3685±0.0048 | 0.3685±0.0048 | 0.3682±0.0048 | 0.3684±0.0048 | 0.3678±0.0048 | 0.3672±0.0047 | 0.3675±0.0048 | 0.3676±0.0048 | 0.3674±0.0047 | 0.3668±0.0047 | 0.366±0.0047 |
| Guizhou | 0.3837±0.005 | 0.3821±0.0049 | 0.3808±0.0049 | 0.3801±0.0049 | 0.3795±0.0049 | 0.3793±0.0049 | 0.3793±0.0049 | 0.3791±0.0049 | 0.3789±0.0049 | 0.379±0.0049 | 0.3786±0.0049 | 0.3782±0.0049 | 0.3784±0.0049 | 0.3784±0.0049 | 0.3783±0.0049 | 0.378±0.0049 | 0.3776±0.0049 |
| Yunnan | 0.3844±0.005 | 0.383±0.0049 | 0.3817±0.0049 | 0.381±0.0049 | 0.3806±0.0049 | 0.3804±0.0049 | 0.3803±0.0049 | 0.3802±0.0049 | 0.3801±0.0049 | 0.3802±0.0049 | 0.3799±0.0049 | 0.3796±0.0049 | 0.3798±0.0049 | 0.3799±0.0049 | 0.3799±0.0049 | 0.3796±0.0049 | 0.3792±0.0049 |
| Tibet | 0.3877±0.005 | 0.3869±0.005 | 0.3862±0.005 | 0.3856±0.005 | 0.3852±0.005 | 0.3851±0.005 | 0.385±0.005 | 0.3849±0.005 | 0.3847±0.005 | 0.3848±0.005 | 0.3846±0.005 | 0.3843±0.005 | 0.3845±0.005 | 0.3846±0.005 | 0.3845±0.005 | 0.3843±0.005 | 0.384±0.005 |
| Shaanxi | 0.3782±0.0049 | 0.376±0.0049 | 0.3743±0.0048 | 0.3728±0.0048 | 0.3719±0.0048 | 0.3714±0.0048 | 0.3712±0.0048 | 0.3711±0.0048 | 0.3708±0.0048 | 0.3709±0.0048 | 0.3704±0.0048 | 0.3699±0.0048 | 0.3703±0.0048 | 0.3705±0.0048 | 0.3701±0.0048 | 0.3698±0.0048 | 0.3691±0.0048 |
| Gansu | 0.3768±0.0049 | 0.3743±0.0048 | 0.3722±0.0048 | 0.3709±0.0048 | 0.3698±0.0048 | 0.3694±0.0048 | 0.3693±0.0048 | 0.3693±0.0048 | 0.3689±0.0048 | 0.3692±0.0048 | 0.3687±0.0048 | 0.3681±0.0048 | 0.3685±0.0048 | 0.3687±0.0048 | 0.3685±0.0048 | 0.368±0.0048 | 0.3673±0.0047 |
| Qinghai | 0.3795±0.0049 | 0.3776±0.0049 | 0.3759±0.0049 | 0.3748±0.0048 | 0.3739±0.0048 | 0.3735±0.0048 | 0.3734±0.0048 | 0.3733±0.0048 | 0.373±0.0048 | 0.3731±0.0048 | 0.3726±0.0048 | 0.3721±0.0048 | 0.3724±0.0048 | 0.3726±0.0048 | 0.3724±0.0048 | 0.3719±0.0048 | 0.3711±0.0048 |
| Ningxia | 0.3806±0.0049 | 0.3787±0.0049 | 0.3771±0.0049 | 0.3761±0.0049 | 0.3753±0.0049 | 0.3751±0.0048 | 0.375±0.0048 | 0.3748±0.0048 | 0.3745±0.0048 | 0.3746±0.0048 | 0.3741±0.0048 | 0.3737±0.0048 | 0.3739±0.0048 | 0.3739±0.0048 | 0.3737±0.0048 | 0.3733±0.0048 | 0.3727±0.0048 |
| Xinjiang | 0.3765±0.0049 | 0.3739±0.0048 | 0.3715±0.0048 | 0.3701±0.0048 | 0.3692±0.0048 | 0.3688±0.0048 | 0.3688±0.0048 | 0.3688±0.0048 | 0.3681±0.0048 | 0.3683±0.0048 | 0.3678±0.0048 | 0.3673±0.0047 | 0.3676±0.0048 | 0.3677±0.0048 | 0.3676±0.0048 | 0.367±0.0047 | 0.3663±0.0047 |

**Table S30.** The estimated misalignment factors across provinces with DeepEnergy.

| Province | 2021-01 | 2021-02 | 2021-03 | 2021-04 | 2021-05 | 2021-06 | 2021-07 | 2021-08 | 2021-09 | 2021-10 | 2021-11 | 2021-12 | 2022-01 | 2022-02 | 2022-03 | 2022-04 | 2022-05 |
|---|---|---|---|---|---|---|---|---|---|---|---|---|---|---|---|---|---|
| Beijing | 0.2438±0.0069 | 0.2416±0.0069 | 0.2398±0.0068 | 0.2386±0.0068 | 0.2378±0.0068 | 0.2374±0.0067 | 0.2373±0.0067 | 0.2371±0.0067 | 0.2368±0.0067 | 0.2371±0.0067 | 0.2364±0.0067 | 0.2358±0.0067 | 0.2363±0.0067 | 0.2366±0.0067 | 0.2366±0.0067 | 0.2361±0.0067 | 0.2354±0.0067 |
| Tianjing | 0.2487±0.0071 | 0.247±0.007 | 0.2456±0.007 | 0.2447±0.0069 | 0.2441±0.0069 | 0.2438±0.0069 | 0.2437±0.0069 | 0.2438±0.0069 | 0.2437±0.0069 | 0.2437±0.0069 | 0.2433±0.0069 | 0.243±0.0069 | 0.2433±0.0069 | 0.2434±0.0069 | 0.2433±0.0069 | 0.2429±0.0069 | 0.2426±0.0069 |
| Hebei | 0.2486±0.0071 | 0.2469±0.007 | 0.2455±0.007 | 0.2446±0.0069 | 0.2439±0.0069 | 0.2437±0.0069 | 0.2436±0.0069 | 0.2435±0.0069 | 0.2433±0.0069 | 0.2434±0.0069 | 0.243±0.0069 | 0.2426±0.0069 | 0.2428±0.0069 | 0.2429±0.0069 | 0.2429±0.0069 | 0.2426±0.0069 | 0.2421±0.0069 |
| Shanxi | 0.2516±0.0071 | 0.2504±0.0071 | 0.2493±0.0071 | 0.2487±0.0071 | 0.2482±0.007 | 0.248±0.007 | 0.248±0.007 | 0.248±0.007 | 0.2478±0.007 | 0.2479±0.007 | 0.2476±0.007 | 0.2473±0.007 | 0.2475±0.007 | 0.2476±0.007 | 0.2475±0.007 | 0.2472±0.007 | 0.2468±0.007 |
| Inner Mongolia | 0.2495±0.0071 | 0.2481±0.007 | 0.2468±0.007 | 0.246±0.007 | 0.2455±0.007 | 0.2453±0.007 | 0.2452±0.007 | 0.2452±0.007 | 0.245±0.007 | 0.2452±0.007 | 0.2447±0.0069 | 0.2443±0.0069 | 0.2446±0.0069 | 0.2447±0.0069 | 0.2446±0.0069 | 0.2443±0.0069 | 0.2438±0.0069 |
| Liaoning | 0.2476±0.007 | 0.2458±0.007 | 0.2443±0.0069 | 0.2433±0.0069 | 0.2426±0.0069 | 0.2424±0.0069 | 0.2423±0.0069 | 0.2423±0.0069 | 0.242±0.0069 | 0.2421±0.0069 | 0.2417±0.0069 | 0.2413±0.0069 | 0.2416±0.0069 | 0.2418±0.0069 | 0.2416±0.0069 | 0.2413±0.0069 | 0.2407±0.0068 |
| Jilin | 0.245±0.007 | 0.2429±0.0069 | 0.2411±0.0068 | 0.2399±0.0068 | 0.239±0.0068 | 0.2387±0.0068 | 0.2386±0.0068 | 0.2386±0.0068 | 0.2383±0.0068 | 0.2385±0.0068 | 0.2378±0.0068 | 0.2373±0.0067 | 0.2376±0.0067 | 0.2378±0.0068 | 0.2378±0.0068 | 0.2375±0.0067 | 0.2367±0.0067 |
| Heilongjiang | 0.2497±0.0071 | 0.2485±0.0071 | 0.2473±0.007 | 0.2466±0.007 | 0.2459±0.007 | 0.2458±0.007 | 0.2458±0.007 | 0.2458±0.007 | 0.2455±0.007 | 0.2456±0.007 | 0.2452±0.007 | 0.2451±0.007 | 0.2453±0.007 | 0.2453±0.007 | 0.2453±0.007 | 0.245±0.007 | 0.2445±0.0069 |
| Shanghai | 0.2482±0.007 | 0.2465±0.007 | 0.245±0.007 | 0.244±0.0069 | 0.2432±0.0069 | 0.2429±0.0069 | 0.2428±0.0069 | 0.2427±0.0069 | 0.2426±0.0069 | 0.2427±0.0069 | 0.2422±0.0069 | 0.2422±0.0069 | 0.2424±0.0069 | 0.2425±0.0069 | 0.2425±0.0069 | 0.2424±0.0069 | 0.2422±0.0069 |
| Jiangsu | 0.2508±0.0071 | 0.2495±0.0071 | 0.2483±0.0071 | 0.2476±0.007 | 0.2471±0.007 | 0.2469±0.007 | 0.2468±0.007 | 0.2468±0.007 | 0.2467±0.007 | 0.2467±0.007 | 0.2464±0.007 | 0.2461±0.007 | 0.2462±0.007 | 0.2463±0.007 | 0.2461±0.007 | 0.2459±0.007 | 0.2455±0.007 |
| Zhejiang | 0.2508±0.0071 | 0.2496±0.0071 | 0.2484±0.0071 | 0.2476±0.007 | 0.247±0.007 | 0.2469±0.007 | 0.2468±0.007 | 0.2467±0.007 | 0.2465±0.007 | 0.2466±0.007 | 0.2463±0.007 | 0.246±0.007 | 0.2462±0.007 | 0.2463±0.007 | 0.2461±0.007 | 0.2458±0.007 | 0.2454±0.007 |
| Anhui | 0.2501±0.0071 | 0.2486±0.0071 | 0.2473±0.007 | 0.2465±0.007 | 0.2459±0.007 | 0.2457±0.007 | 0.2456±0.007 | 0.2456±0.007 | 0.2454±0.007 | 0.2456±0.007 | 0.2452±0.007 | 0.245±0.007 | 0.2451±0.007 | 0.2451±0.007 | 0.2451±0.007 | 0.2448±0.007 | 0.2443±0.0069 |
| Fujian | 0.2522±0.0072 | 0.2511±0.0071 | 0.2501±0.0071 | 0.2494±0.0071 | 0.249±0.0071 | 0.2488±0.0071 | 0.2488±0.0071 | 0.2487±0.0071 | 0.2486±0.0071 | 0.2487±0.0071 | 0.2484±0.0071 | 0.2482±0.007 | 0.2484±0.0071 | 0.2485±0.0071 | 0.2484±0.0071 | 0.2482±0.007 | 0.2478±0.007 |
| Jiangxi | 0.2535±0.0072 | 0.2524±0.0072 | 0.2515±0.0071 | 0.251±0.0071 | 0.2506±0.0071 | 0.2504±0.0071 | 0.2503±0.0071 | 0.2502±0.0071 | 0.2501±0.0071 | 0.2501±0.0071 | 0.25±0.0071 | 0.2497±0.0071 | 0.2497±0.0071 | 0.2496±0.0071 | 0.2496±0.0071 | 0.2495±0.0071 | 0.2495±0.0071 |
| Shandong | 0.2491±0.0071 | 0.2475±0.007 | 0.2461±0.007 | 0.2453±0.007 | 0.2446±0.0069 | 0.2444±0.0069 | 0.2443±0.0069 | 0.2442±0.0069 | 0.2441±0.0069 | 0.2441±0.0069 | 0.2437±0.0069 | 0.2434±0.0069 | 0.2436±0.0069 | 0.2436±0.0069 | 0.2435±0.0069 | 0.2431±0.0069 | 0.2425±0.0069 |
| Henan | 0.2445±0.0069 | 0.2421±0.0069 | 0.2402±0.0068 | 0.239±0.0068 | 0.2381±0.0068 | 0.2378±0.0068 | 0.2377±0.0067 | 0.2377±0.0068 | 0.2375±0.0067 | 0.2376±0.0067 | 0.237±0.0067 | 0.2366±0.0067 | 0.2369±0.0067 | 0.237±0.0067 | 0.2368±0.0067 | 0.2364±0.0067 | 0.2357±0.0067 |
| Hubei | 0.2515±0.0071 | 0.2502±0.0071 | 0.249±0.0071 | 0.2484±0.0071 | 0.2479±0.007 | 0.2477±0.007 | 0.2477±0.007 | 0.2476±0.007 | 0.2474±0.007 | 0.2475±0.007 | 0.2472±0.007 | 0.247±0.007 | 0.2471±0.007 | 0.2472±0.007 | 0.2471±0.007 | 0.2468±0.007 | 0.2465±0.007 |
| Hunan | 0.2486±0.0071 | 0.2468±0.007 | 0.2455±0.007 | 0.2446±0.0069 | 0.2438±0.0069 | 0.2436±0.0069 | 0.2435±0.0069 | 0.2435±0.0069 | 0.2432±0.0069 | 0.2434±0.0069 | 0.243±0.0069 | 0.2427±0.0069 | 0.243±0.0069 | 0.2431±0.0069 | 0.243±0.0069 | 0.2427±0.0069 | 0.2422±0.0069 |
| Guangdong | 0.2489±0.0071 | 0.2474±0.007 | 0.246±0.007 | 0.245±0.007 | 0.2444±0.0069 | 0.2441±0.0069 | 0.244±0.0069 | 0.2439±0.0069 | 0.2436±0.0069 | 0.2437±0.0069 | 0.2433±0.0069 | 0.2429±0.0069 | 0.2431±0.0069 | 0.2432±0.0069 | 0.2429±0.0069 | 0.2425±0.0069 | 0.242±0.0069 |
| Guangxi | 0.2475±0.007 | 0.2456±0.007 | 0.244±0.0069 | 0.2431±0.0069 | 0.2424±0.0069 | 0.2422±0.0069 | 0.2421±0.0069 | 0.242±0.0069 | 0.2418±0.0069 | 0.2419±0.0069 | 0.2415±0.0069 | 0.2411±0.0068 | 0.2413±0.0069 | 0.2414±0.0069 | 0.2411±0.0068 | 0.2407±0.0068 | 0.2401±0.0068 |
| Hainan | 0.2504±0.0071 | 0.2491±0.0071 | 0.2478±0.007 | 0.2471±0.007 | 0.2465±0.007 | 0.2464±0.007 | 0.2464±0.007 | 0.2465±0.007 | 0.2461±0.007 | 0.2461±0.007 | 0.2458±0.007 | 0.2455±0.007 | 0.2458±0.007 | 0.2459±0.007 | 0.2456±0.007 | 0.2455±0.007 | 0.2452±0.007 |
| Chongqing | 0.2518±0.0072 | 0.2505±0.0071 | 0.2495±0.0071 | 0.2489±0.0071 | 0.2484±0.0071 | 0.2482±0.007 | 0.2482±0.007 | 0.2481±0.007 | 0.2479±0.007 | 0.248±0.007 | 0.2477±0.007 | 0.2475±0.007 | 0.2476±0.007 | 0.2476±0.007 | 0.2475±0.007 | 0.2472±0.007 | 0.2469±0.007 |
| Sichuan | 0.2484±0.0071 | 0.2466±0.007 | 0.2452±0.007 | 0.2444±0.0069 | 0.2437±0.0069 | 0.2434±0.0069 | 0.2433±0.0069 | 0.2433±0.0069 | 0.2432±0.0069 | 0.2433±0.0069 | 0.2429±0.0069 | 0.2425±0.0069 | 0.2427±0.0069 | 0.2428±0.0069 | 0.2426±0.0069 | 0.2422±0.0069 | 0.2417±0.0069 |
| Guizhou | 0.2534±0.0072 | 0.2524±0.0072 | 0.2515±0.0071 | 0.251±0.0071 | 0.2506±0.0071 | 0.2505±0.0071 | 0.2505±0.0071 | 0.2503±0.0071 | 0.2502±0.0071 | 0.2503±0.0071 | 0.25±0.0071 | 0.2498±0.0071 | 0.2499±0.0071 | 0.2499±0.0071 | 0.2498±0.0071 | 0.2496±0.0071 | 0.2493±0.0071 |
| Yunnan | 0.2539±0.0072 | 0.2529±0.0072 | 0.2521±0.0072 | 0.2516±0.0071 | 0.2513±0.0071 | 0.2512±0.0071 | 0.2512±0.0071 | 0.2511±0.0071 | 0.251±0.0071 | 0.2511±0.0071 | 0.2509±0.0071 | 0.2507±0.0071 | 0.2508±0.0071 | 0.2509±0.0071 | 0.2509±0.0071 | 0.2507±0.0071 | 0.2505±0.0071 |
| Tibet | 0.2561±0.0073 | 0.2555±0.0073 | 0.2551±0.0072 | 0.2546±0.0072 | 0.2544±0.0072 | 0.2543±0.0072 | 0.2542±0.0072 | 0.2542±0.0072 | 0.2541±0.0072 | 0.2541±0.0072 | 0.254±0.0072 | 0.2538±0.0072 | 0.2539±0.0072 | 0.254±0.0072 | 0.2539±0.0072 | 0.2538±0.0072 | 0.2536±0.0072 |
| Shaanxi | 0.2498±0.0071 | 0.2483±0.0071 | 0.2472±0.007 | 0.2462±0.007 | 0.2456±0.007 | 0.2453±0.007 | 0.2451±0.007 | 0.2451±0.007 | 0.2449±0.007 | 0.245±0.007 | 0.2446±0.0069 | 0.2443±0.0069 | 0.2445±0.0069 | 0.2447±0.0069 | 0.2444±0.0069 | 0.2442±0.0069 | 0.2438±0.0069 |
| Gansu | 0.2488±0.0071 | 0.2472±0.007 | 0.2458±0.007 | 0.2449±0.007 | 0.2442±0.0069 | 0.244±0.0069 | 0.2439±0.0069 | 0.2439±0.0069 | 0.2437±0.0069 | 0.2438±0.0069 | 0.2435±0.0069 | 0.2431±0.0069 | 0.2434±0.0069 | 0.2435±0.0069 | 0.2434±0.0069 | 0.2431±0.0069 | 0.2426±0.0069 |
| Qinghai | 0.2506±0.0071 | 0.2494±0.0071 | 0.2483±0.007 | 0.2475±0.007 | 0.2469±0.007 | 0.2467±0.007 | 0.2466±0.007 | 0.2465±0.007 | 0.2463±0.007 | 0.2464±0.007 | 0.246±0.007 | 0.2457±0.007 | 0.246±0.007 | 0.2461±0.007 | 0.2459±0.007 | 0.2456±0.007 | 0.2451±0.007 |
| Ningxia | 0.2514±0.0071 | 0.2501±0.0071 | 0.249±0.0071 | 0.2484±0.0071 | 0.2479±0.007 | 0.2477±0.007 | 0.2476±0.007 | 0.2475±0.007 | 0.2473±0.007 | 0.2474±0.007 | 0.2471±0.007 | 0.2468±0.007 | 0.2469±0.007 | 0.2469±0.007 | 0.2468±0.007 | 0.2465±0.007 | 0.2461±0.007 |
| Xinjiang | 0.2486±0.0071 | 0.2469±0.007 | 0.2454±0.007 | 0.2444±0.0069 | 0.2438±0.0069 | 0.2436±0.0069 | 0.2436±0.0069 | 0.2435±0.0069 | 0.2431±0.0069 | 0.2433±0.0069 | 0.2429±0.0069 | 0.2425±0.0069 | 0.2428±0.0069 | 0.2428±0.0069 | 0.2428±0.0069 | 0.2424±0.0069 | 0.2419±0.0069 |

**Table S31.** The performance of the models trained on data from different regions in Nanchang.

| Models | Energy-saving rate of the whole Nanchang |
|---|---|
| Trained on Region A | 0.4295 |
| Trained on Region B | 0.4482 |
| Trained on Region C | 0.4492 |
| Trained on Region D | 0.4252 |
| Trained on the whole Nanchang | 0.4373 |

**Table S32.** Linear regression analysis for misalignment factor of DeepEnergy models trained on different regions.

| **Linear regression model:** $M = K_{\psi}(1 - \tilde{L})$ | | |
|---|---|---|
| **Dependent variable** | | |
| Normalized network traffic load $\tilde{L}$ | | |
| **DeepEnergy models** | $K_{\psi}$ | $R^2$ |
| DeepEnergy model trained on Region A | 0.2885 | 0.8351 |
| DeepEnergy model trained on Region B | 0.2863 | 0.9092 |
| DeepEnergy model trained on Region C | 0.2661 | 0.8085 |
| DeepEnergy model trained on Region D | 0.2895 | 0.8750 |
| DeepEnergy model trained on the whole Nanchang | 0.2606 | 0.8227 |
